# Supplementary material for: Modeling high-entropy transition-metal alloys with alchemical compression
Source: arXiv:2212.13254 source file (2023-04-07)
Supplement: Supplementary file 1 [file si.pdf]

# Modeling high-entropy transition-metal alloys with alchemical compression
## Supporting Materials

Nataliya Lopanitsyna,[1] Guillaume Fraux,[1] Maximilian A. Springer,[2] Sandip De,[2] and Michele Ceriotti[1]
[1)] *Laboratory of Computational Science and Modeling, Institute of Materials, École Polytechnique Fédérale de Lausanne, 1015 Lausanne, Switzerland*
[2)] *BASF SE, Carl-Bosch-Straße 38, 67056 Ludwigshafen, Germany*

## I. COMPUTATIONAL DETAILS

### A. Electronic structure details

All the reference energies and forces are computed using density-functional theory (DFT), as implemented in the VASP code[1], with the PBESol exchange-correlation functional[2]. The core electrons are treated implicitly using projector augmented wave (PAW) pseudopotentials[3]. We choose conservative values for the convergence parameters of the electronic structure calculation, setting the cutoff for the plane-waves expansion of the wave-function to 550 eV, which is more than 50% larger than largest recommended value across all the elements we considered, and the Brillouin zone sampling uses a $\Gamma$ centered Monkhorst-Pack scheme[4] with an interval between k-points along reciprocal lattice vector 0.04 $\pi$ Å$^{-1}$. To support the choice of k-point denisty, we show below the convergence of the cohesive energy difference levelled against corresponding the most converged calculation (k-point density of 0.025 $\pi$Å$^{-1}$) for four representative structures from the dataset as a function of k-point grid density.

As we mentioned in the main text, all the calculations for the HEA25 dataset were performed with non-polarized DFT. We recalculated a small data set containing 944 FCC ideal crystal structures in order to assess the effects of selecting a different level of theory. The discrepancy on energies and forces amounts to 7 meV/at. MAE, 14 meV/at. RMSE, and 38 meV/Å MAE, 91 meV/Å RMSE correspondingly, which is comparable with the accuracy of the ML model.

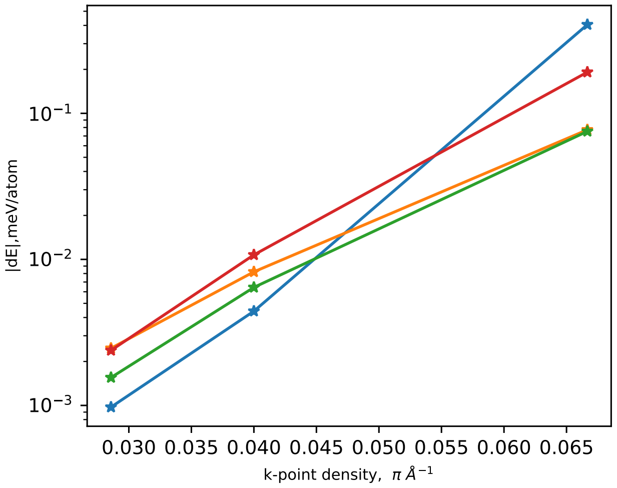


Figure S1. The convergence of the difference in cohesive energy relative to the most converged structure (k-point density of 0.025 $\pi$Å$^{-1}$), for four representative structures in the data set.

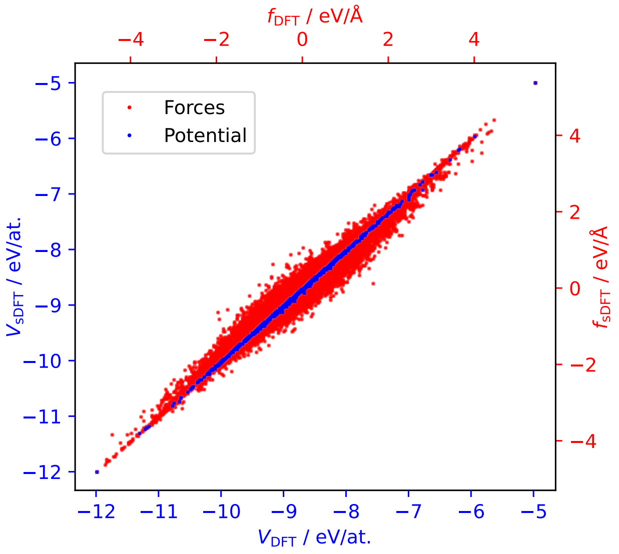


Figure S2. Parity plot between energies and forces computed with spin polarization (sDFT) and without (DFT, level of theory used in the article). The values were compute on a separate dataset of 944 structures. Energy error: 7 meV/at. MAE, 14 meV/at. RMSE, Force error: 38 meV/Å MAE, 91 meV/Å RMSE.

### B. ML Details

In this section, we report the details of the HEA25-4-NN model. The final model HEA25-4-NN includes an atomic-energy baseline (25 weights), linear regression based on 2-body and 3-body correlation features (7500 and 1936 weights respectively), and a multi-layer perceptron with 80-nodes hidden layers (161521 weights, mostly associated with the initial linear layer that compresses the 2 and 3-body weights down to 80 channels). As the result of the alchemical compression with four pseudo-elements, the feature vector size decreases from the original 75625 to 1936. We use a training set containing energies from 25k structures ($N_E$) and forces from 2k structures ($N_F$) and a hold-out testing set containing 500 structures with energies and forces.The loss function is expressed as:

$$\mathcal{L} = \frac{1}{N_E}\sum_{n}^{N_E}\left(\hat{E}_n - E_n\right)^2 + \frac{C_F}{N_F}\sum_{i=1}^{N_F \cdot I_F}\sum_{\alpha=1}^{3}\left(\hat{F}_{i,\alpha} - F_{i,\alpha}\right)^2 + \lambda_1||w_1|| + \lambda_2||w_2|| + \lambda_3||w_3|| + \lambda_{NN}\sum||w_{NN}||, \quad (1)$$

where $\hat{E}_n$ and $E_n$ are predicted and reference energies, $\hat{F}_{i,\alpha}$ and $F_{i,\alpha}$ predicted and reference forces, $I$ the total number of atoms for which forces are considered in training, $C_F$ is a scaling factor set to 1e−3, $\lambda_{1,2,3,NN}$ (respectively $w_{1,2,3,NN}$) are the regularizers (respectively weight matrices) for the linear 1 (aeb), 2, 3-body, and NN models. These regularizers are set to $10^{-4}$ for $\lambda_{1,2,3}$ and $10^{-2}$ for $\lambda_{NN}$

For two-body and three-body representations, we use GTO basis functions and radial scaling following Ref. 5. Table I presents the hyper-parameters used in the HEA25-4-NN. The model weights (best.torch) and it's parameters (parameters.json) are provided in the Supplementary Materials.

| | two-body | three-body |
|---|---|---|
| $\sigma_w$/Å | 0.25 | 0.3 |
| $r_{cut}$/Å | 6.0 | 5.0 |
| $n_{\text{alch}}$ | | 4 |
| $n_{max}, l_{max}$ | 12 | $8, 4^*$ |

Table I. Key hyper-parameters of the HEA25-4-NN model. Here $\sigma_w$ is the Gaussian width, $r_{cut}$ – the cutoff radius, $n_{\text{alch}}$ – the number of alchemical channels,$n_{max}$ and $l_{max}$ – the number of radial and angular channels. For the three-body representation we used a different number of radial channels for every $l$. The complete set of parameters can be found in the parameters.json file, which is provided in the Supplementary Materials.

## II. ALCHEMICAL CONTRACTION

### A. Weight analysis

We continue the analysis of the alchemical compression by demonstrating the evolution of the alchemical weights matrix $\mathbf{u}_{\mathrm{alch}}$ during the optimization process(Fig. S3). Despite initializing the weights of $\mathbf{u}_{\mathrm{alch}}$ with physical priors - a singular value decomposition of a Gaussian similarity kernel based on electronegativity and atomic radius of the elements, as in Ref. 5 - one does not observe a clear arrangement of the elements according to their positions in the $d$ block (Fig. S3, left panel). Some elements are projected in the vicinity of their conventional periodic table neighbours, while others such as Mn are grouped with dissimilar elements.

Conversely, the optimized weight for the HEA25-4-NN potential (Fig. S3, right panel, corresponding to the figure in the main text) are clearly laid out as in a distorted version of the transition metal block. This regular arrangement is obtained in both the HEA25-4-NN model and in the linear models, as shown in Fig. S4. With the exception of $\mathbf{n}_{\mathrm{alch}} = 2$ (where the excessive compression leads to an irregular distribution) the optimized weight reflect the position of the elements in the periodic table. Furthermore, the comparison of the explained variance's plots for linear models (Fig. S5), confirms that for the optimized weights the first three components carry the most information about chemical diversity for the chosen set of elements.

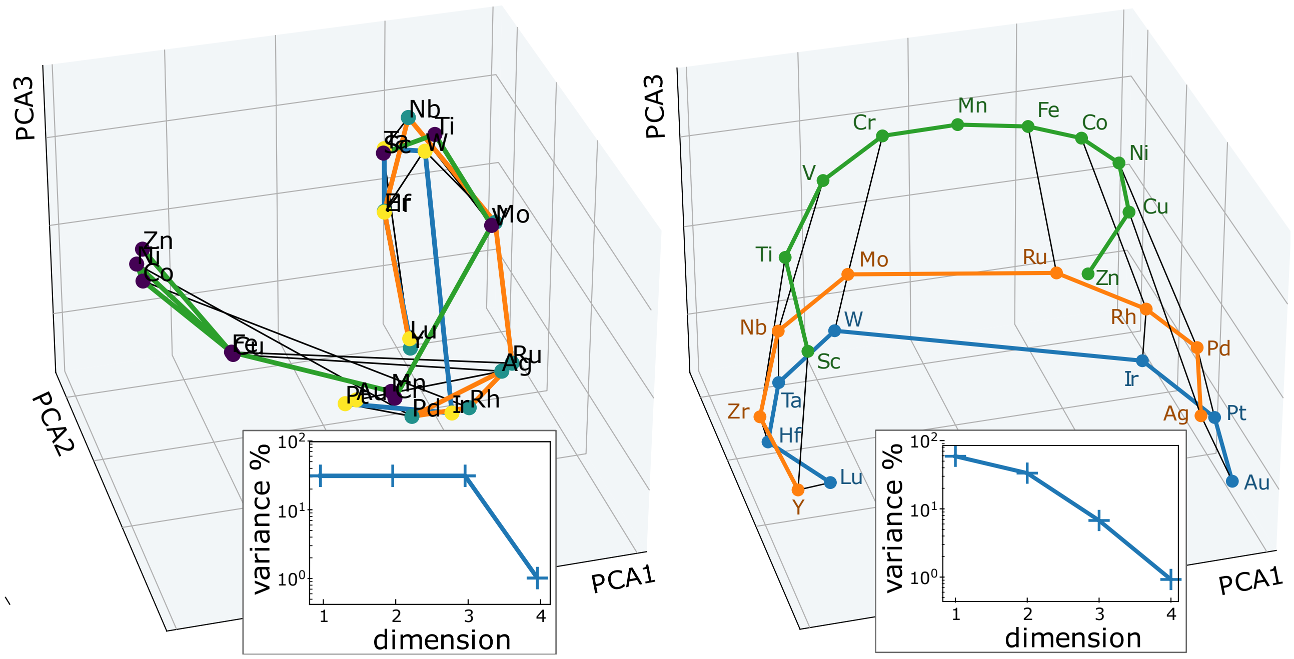


Figure S3. Top-3 principal components of the initial (left) and converged (right) alchemical weights matrix $\mathbf{u}_{\mathrm{alch}}$ for the HEA25-4-NN model. The periods are highlighted with orange, blue and green lines, and the columns are indicated by black thin lines. The insets show the decay of explained variance with number of alchemical channels

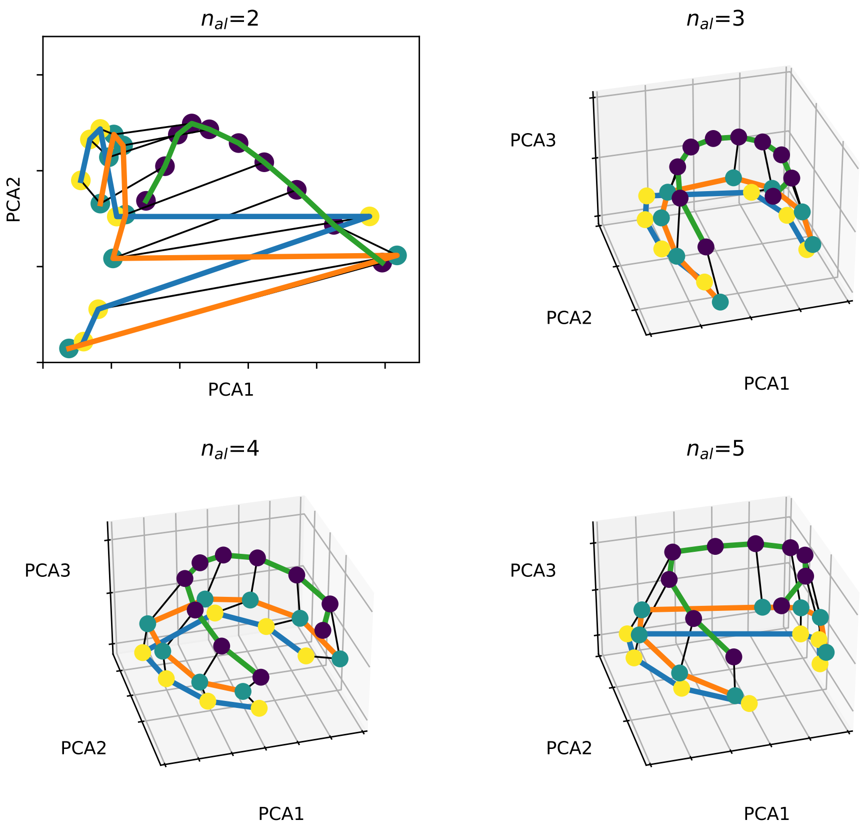


Figure S4. Comparison of converged alchemical weights matrices $\mathbf{u}_{\text{alch}}$ for different number of alchemical channels ( $\mathbf{n}_{\text{alch}} = 2, 3, 4, 5$) represented in principal components space for the $V^{(\text{aeb})} + V^{(\text{3B})}$ models. The periods are highlighted with orange, blue and green lines, and the columns are indicated by black thin lines.

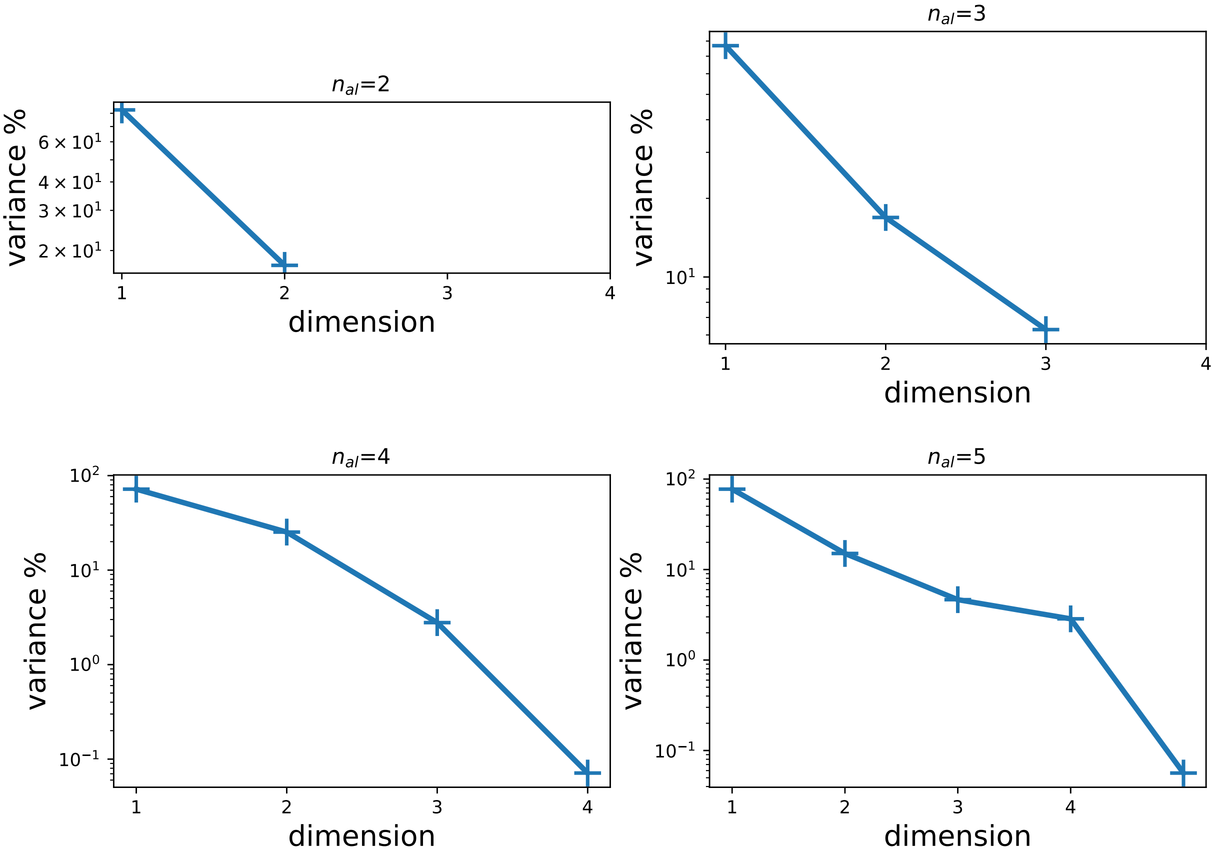


Figure S5. Comparison of the decay of the explained variance for a different number of alchemical channels ( $\mathbf{n}_{\mathrm{alch}} = 2, 3, 4, 5$) represented in principal components space for the $V^{(\mathrm{aeb})} + V^{(3\mathrm{B})}$ models.

### B. Alchemical interpolation

Exploiting the interpretability of the alchemical weights, we interpolated linearly the weights for not represented elements Re and Os, as discussed in the main text. We determined the weights for $V^{(\mathrm{aeb})}$ (that are not contracted) by fitting the residual errors with a two-parameter model. Here we provide a parity plot between reference and predicted energies for a clearer picture (Fig. S6).

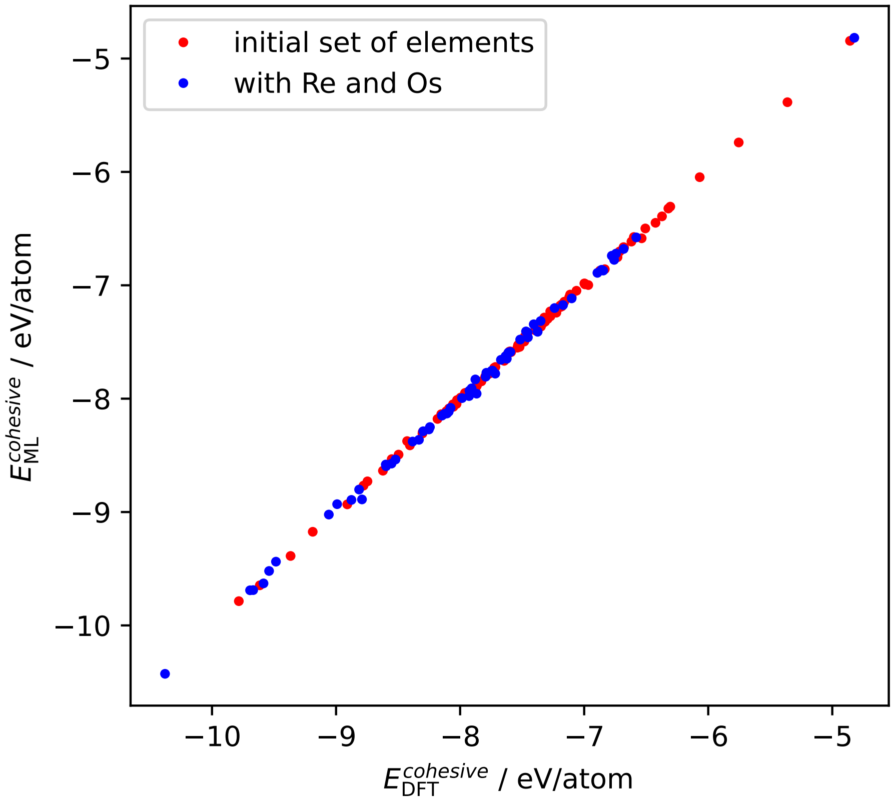


Figure S6. Parity plot between energies computed with DFT and predicted with the $n_{\mathrm{alch}} = 4$ $V^{(\mathrm{aeb})} + V^{(\mathrm{3B})}$ model. In red are depicted the points corresponding to 60 structures from the hold-out fraction of HEA25 dataset. We randomly substituted some atoms with Re and Os, re-computed the corresponding energies with DFT and predicted energies interpolating the weights linearly from the $V^{(\mathrm{aeb})} + V^{(\mathrm{3B})}$ alchemical coupling matrix. The resulting energies are plotted as blue points.

## III. VALIDATION

### A. Binary Convex Hull

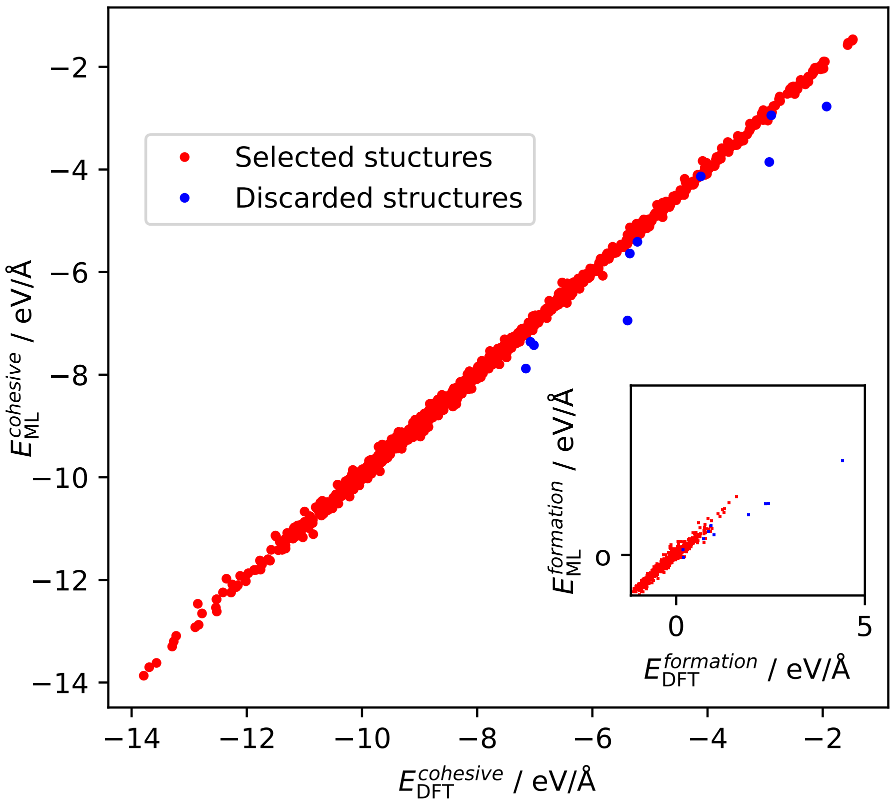


Figure S7. Parity plots between cohesive energies and formation energies (in the inset) computed with DFT and predicted with HEA25-4-NN (ML). Used in the analysis data points are depicted in red, and discarded structures – in blue.

As the HEA dataset contains only structures based on BCC and FCC crystalline lattices, for a descriptive evaluation of HEA25-4-NN performance, we discarded 10 structures out of 1415 which were too dissimilar from BCC or FCC. To measure the similarity, we computed the minimum Euclidean distance in the top-10 principle component space of power spectrum features to FCC or BCC ideal crystals ($\mathrm{P}^{\mathrm{FCC}}$,$\mathrm{P}^{\mathrm{BCC}}$ ) for each binary structure ($\mathrm{P}^{\mathrm{i}}$) as defined in (2). Fig. S8 illustrates the correlation between the introduced distance and the absolute difference in cohesive energies between DFT and HEA25-4-NN predictions. We set a threshold of 40, past which the structures were not considered (in blue). All the structures labeled in red were used to compute the MAE for the figures here and in the main text. The parity plot in Fig. S7 preserves the same colour scheme and demonstrates that all the outliers belong to the group of structures that bear no resemblance to those included in the HEA training dataset.

$$\text{dist.} = \min\{d[PCA_{10}(P^i), PCA_{10}(P^{FCC})], d[PCA_{10}(P^i), PCA_{10}(P^{BCC})]\}. \quad (2)$$

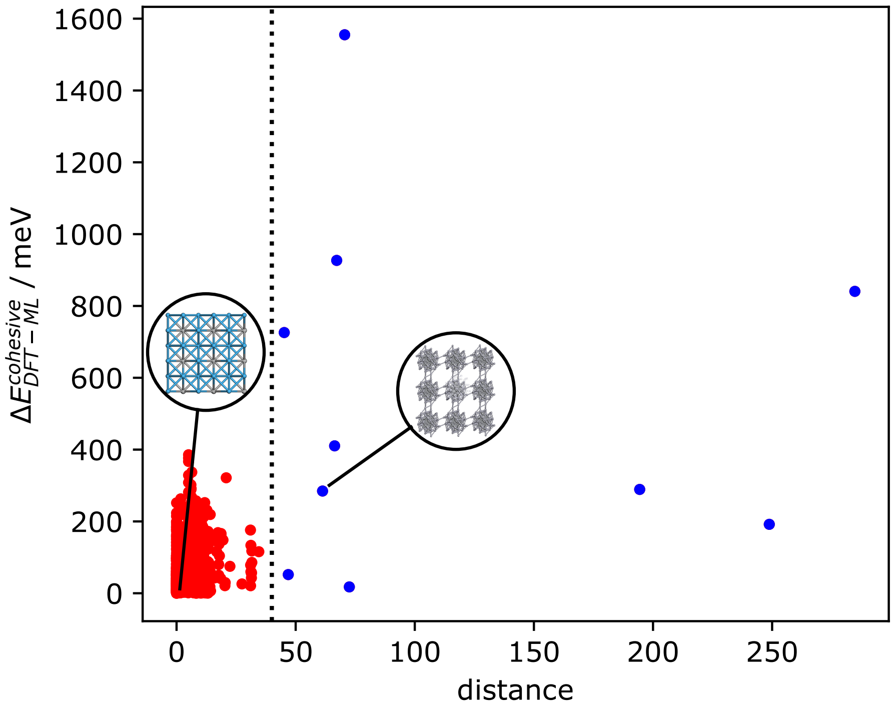


Figure S8. Correlation plot between the absolute difference in cohesive energies between DFT and HEA25-4-NN predictions and distance computed in principle component space of power spectrum features reflecting the similarity of each structure to FCC or BCC phases. The dashed vertical line, set at 40, indicates the threshold above which we discarded structures as outliers (in blue).

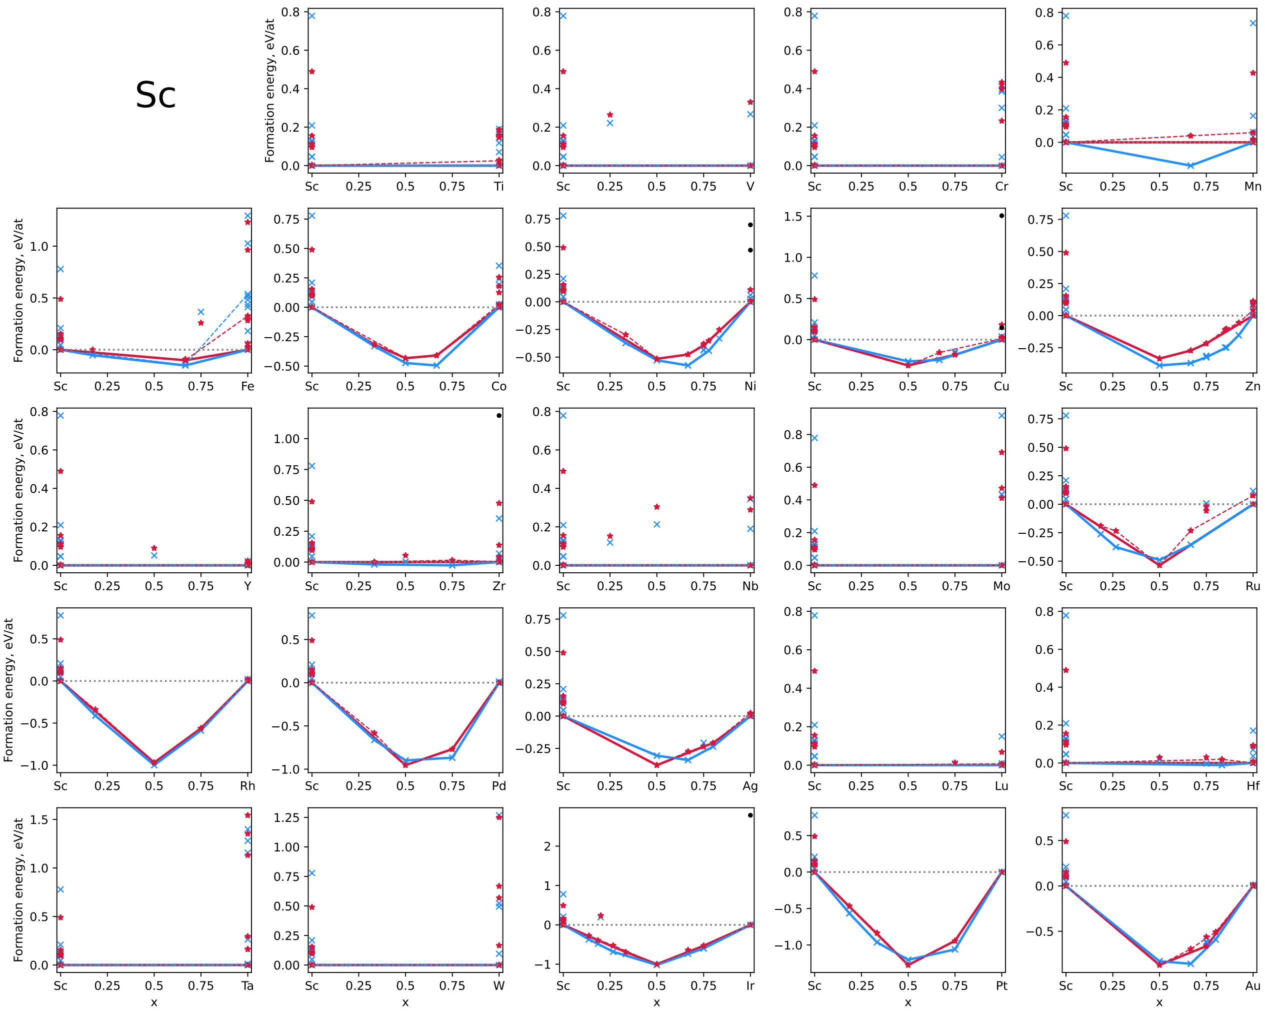


Figure S9. Hull plots for all possible pairs available within the HEA dataset with Sc. Solid lines highlight the hulls obtained from the single-point DFT calculations (blue) and the ML predictions (purple). The dashed line identifies the structures that are stable based on the energies available in the Materials Project database. Black points reflect discarded structures based on the distance measure reflecting the similarity to BCC or FCC phases. The full list of convex hulls is included the very end of this document in Sec. VI

### B. Reference results with M3GNet

We report here result obtained with M3GNet[6], a universal force-field trained on DFT data. We found the energies predicted by M3GNet to be offset from our DFT calculations by a constant factor of -438 meV/atom, which we correct for in the figures below. The error on the validation set is 15 times larger than that of HEA25-4-NN for the energy, and 2 times larger for the forces, and in almost every test we consider the error of M3GNet is much higher than that of HEA25-4-NN. It is important to consider that M3GNet targets an even broader portion of the periodic table, and that its training set of M3GNet is computed with different DFT details than ours, and so part of the error might be due to this discrepancy.

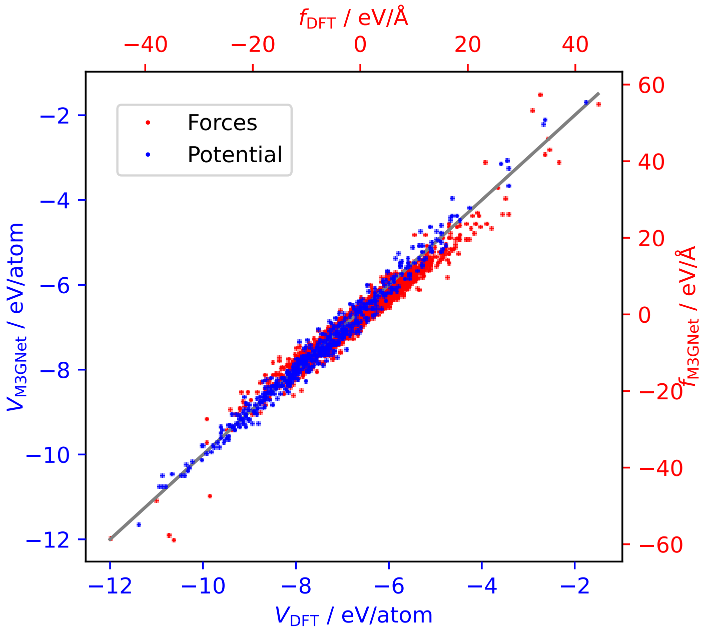


Figure S10. Comparison between the potential energy evaluated by M3GNet and DFT for the 500 hold-out structures used in the main text. A constant offset of -438 meV/atom has been applied to remove the constant shift in predicted energies compared to DFT. The energy MAE is 158 meV/atom, and the force MAE is 387 meV/Å.

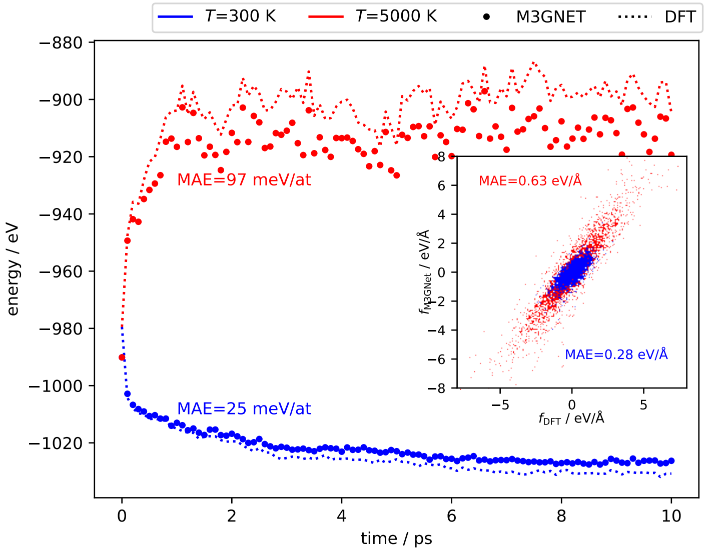


Figure S11. Comparison between the potential energy evaluated by M3GNet and DFT for the 100 snapshots of the same trajectories used in the main text. A constant offset of -438 meV/atom has been applied to remove the constant shift in predicted energies compared to DFT. The inset shows a parity plot for the force components computed for those structures. Energies have a MAE of 25 (97) meV/atom and forces a component MAE of 0.28 (0.63) eV/ Å for the 300 (5000) K trajectory.

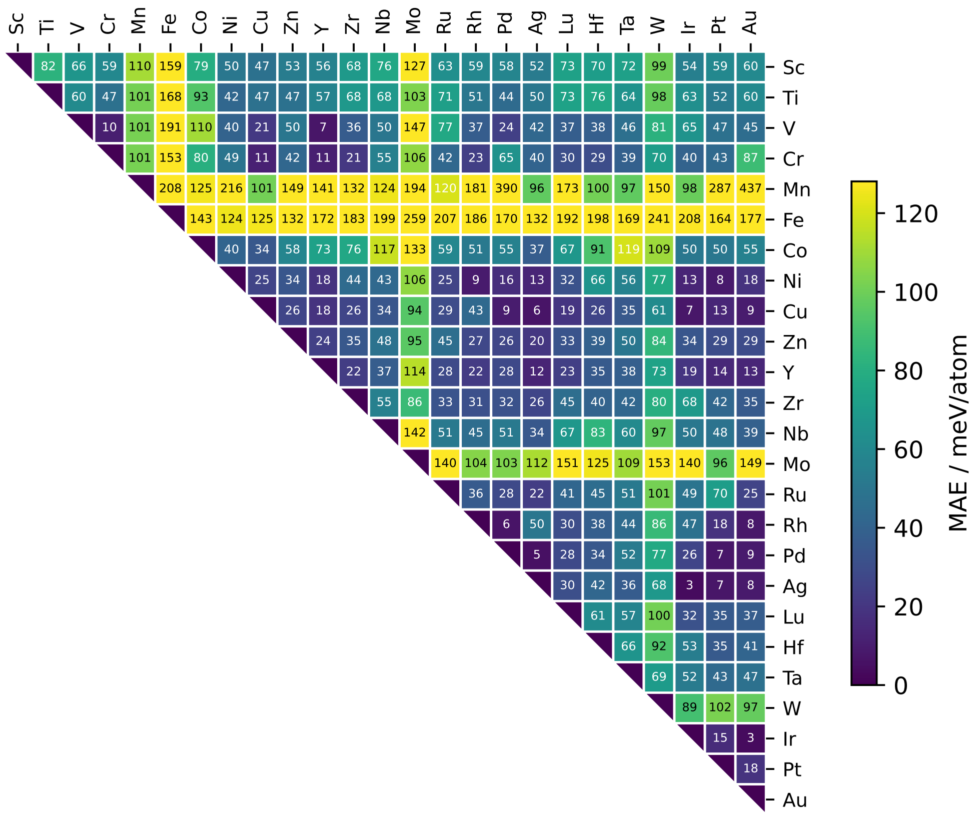


Figure S12. MAE for the formation energy of binary compounds from the Materials Project database as predicted by M3GNet, similar to the corresponding figure in the main text.

## IV. CONVERGENCE OF SIMULATIONS FOR THE $HEA_{all}$ SYSTEM

As discussed in the main text, it is a challenge to converge the simulations for the $HEA_{all}$ system, and even the REMD/MC accelerated-sampling setup we use is not able to reach a plateau for the potential energy of the system. It is also important to consider the impact of finite-size effects on the results of the simulations: a too small simulation cell may prevent precipitation as there are not enough atoms to form a critical nucleus.

### A. Equilibration

In order to verify that finite simulation length does not affect the qualitative observations we make on the affinity between the different elements, we perform simulations with a smaller box containing 125 atoms, that is both faster to run and easier to equilibrate, thanks to finite-size effects that prevent the formation of clear-cut separate phases. Fig. S13 shows that even for this smaller box, and for 500'000 REMD/MC steps (amounting to 16 million energy evaluations) energy is not fully converged.

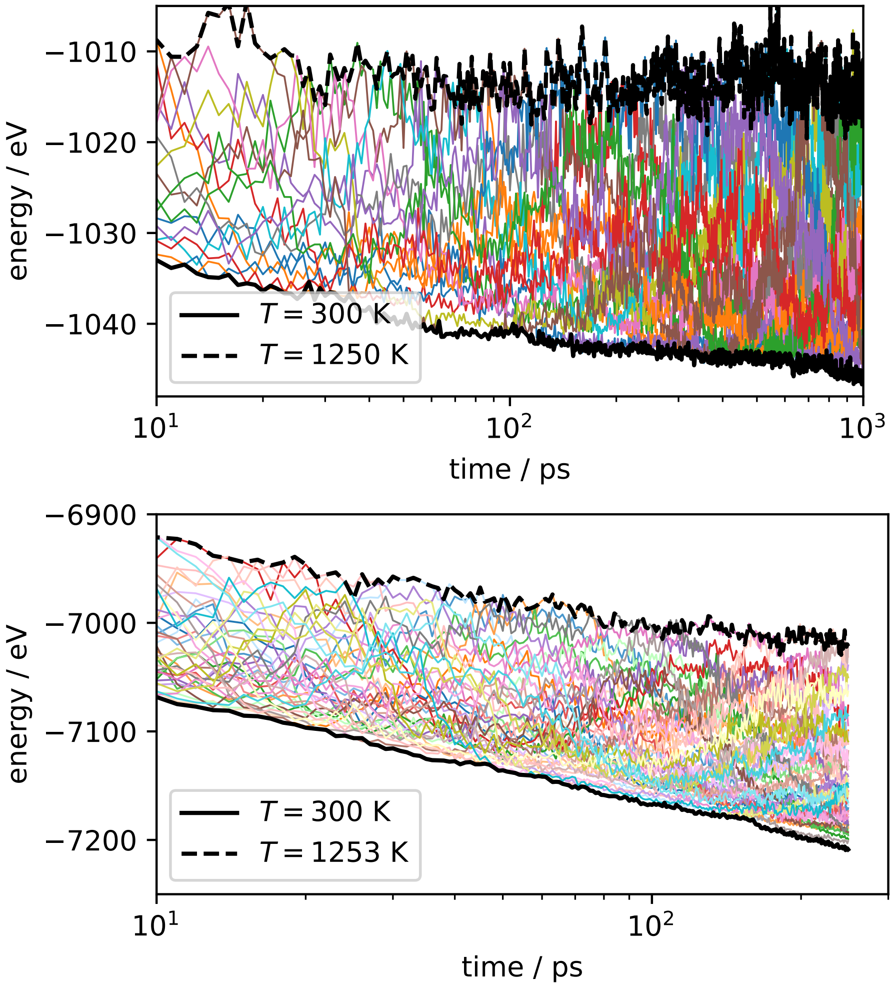


Figure S13. Trajectories of the potential energy for the $HEA_{all}$ system with a 125-atoms box (top) compared with a 864-atoms box (bottom). The different trajectories correspond to 16 (40) replicas evolving with a combination of MD/MC steps, and parallel-tempering energy exchanges. The time scale refers to the MD integration time.

However, pair correlation functions are well-defined and weakly dependent on the starting conditions (Fig. S14). As a consequence, also the RPPs computed for the six independent trajectories are qualitatively in agreement, although they differ by as much as 0.5 units for the low-temperature replicas. High-temperature results are instead very consistent, with discrepancies below 0.05 units.

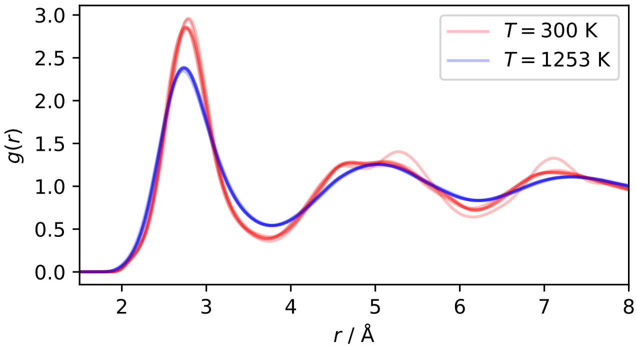


Figure S14. Plots of the total pair correlation function for the low (300 K) and high (1253 K) replicas of a REMD/MC simulation of a 125-atoms box of $HEA_{all}$. The lines correspond to six independent runs, each 1 ns long, with the first 100 ps discarded for (pre)-equilibration.

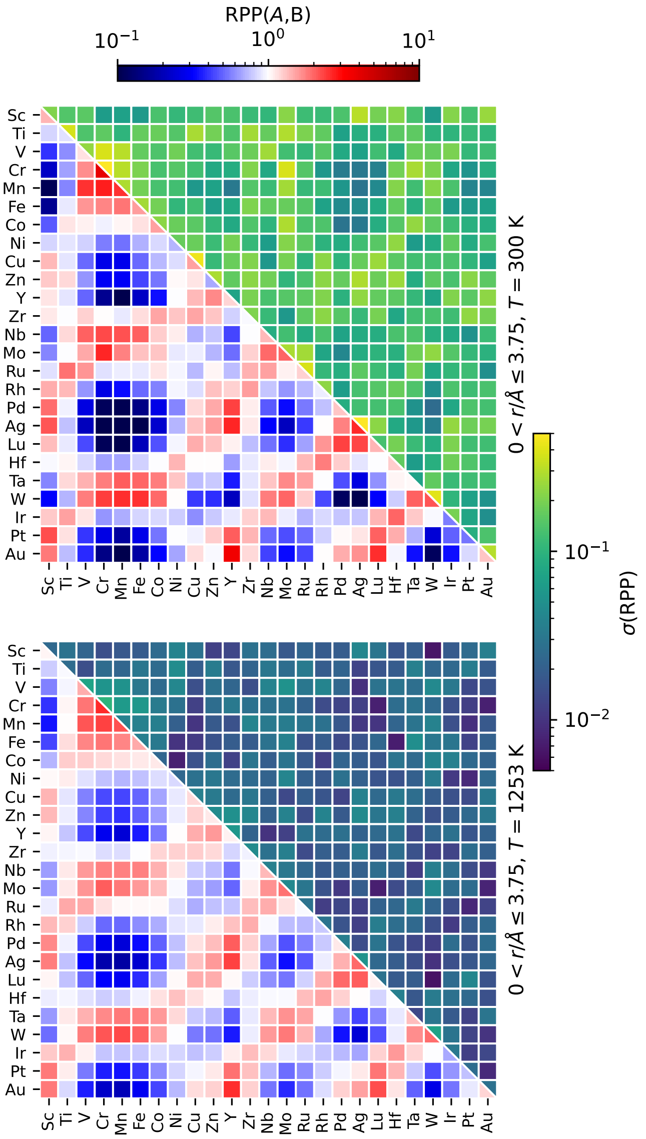


Figure S15. Short-range relative pair probabilities for a 125-atoms box of $HEA_{all}$, obtained by averaging 6 independent trajectories. The upper-right corner of each panel shows the standard deviation of the RPPs between the 6 trajectories.

### B. Finite-size effects

Comparing Fig. IV B with the corresponding figure in the main text, one sees that using a smaller box does not affect the short-range order, with the RPP in the first neighbor shell being equal within the statistical uncertainty to that computed for the larger supercell. On the other hand, one sees clearly the presence of finite-size effects in the third neighbor shell: whereas the 864-atoms cell shows that the long-range affinity of species is weaker than, but correlated to, the short-range RPPs, in the 125-atoms box one observes almost perfect anti-correlation. This is an artifact due to the small number of atoms present in the box, that leads to depletion of the species that cluster together strongly.

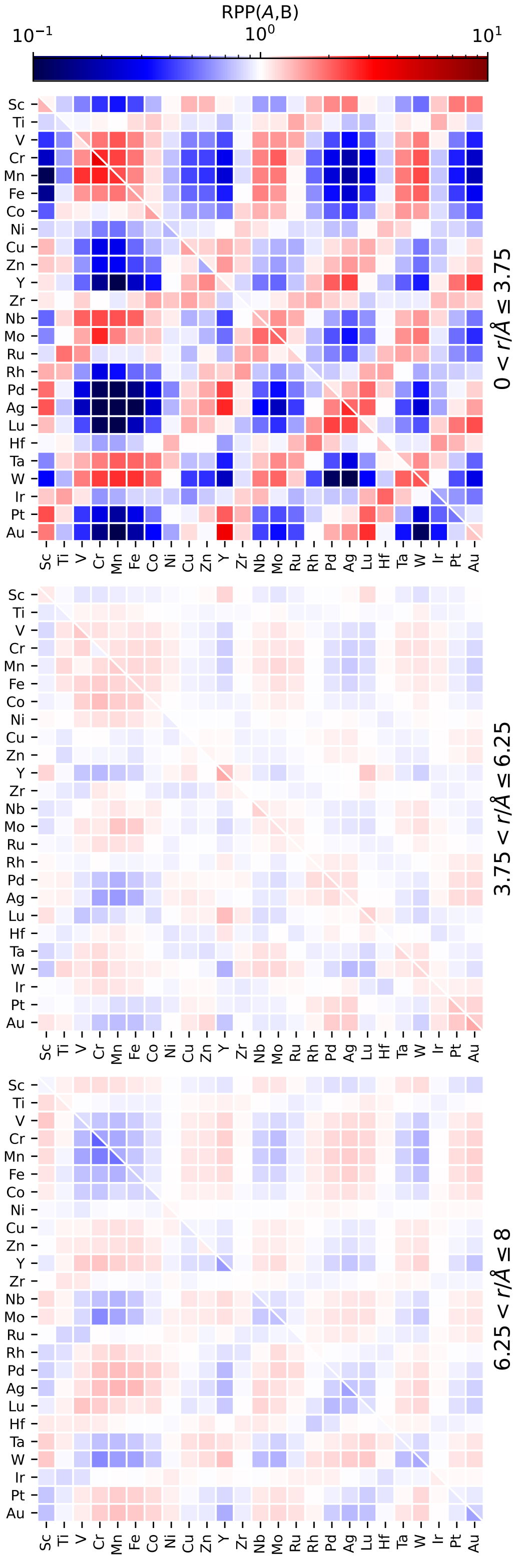


Figure S16. A plot of the relative pair probability for all atom pairs and the three regions corresponding to the first, second, and third peaks in the total pair correlation function. Each plot shows results for a 125-atoms simulations of $HEA_{all}$ at both 300 K (lower-left corner) and 1253 K (top-right corner), averaged over the trajectories and discarding the first 100 ps (50'000 combined MD/MC steps).

## V. FURTHER INFORMATION ON SIMULATIONS OF HIGH-ENTROPY ALLOYS FOR CATALYSIS

For each of the three compositions we consider we show the pair correlation functions at $T = 300$ K and $T = 1253$ K, and the RPPs at the two temperatures and for three ranges of distances.

### A. CoCrFeMnNi

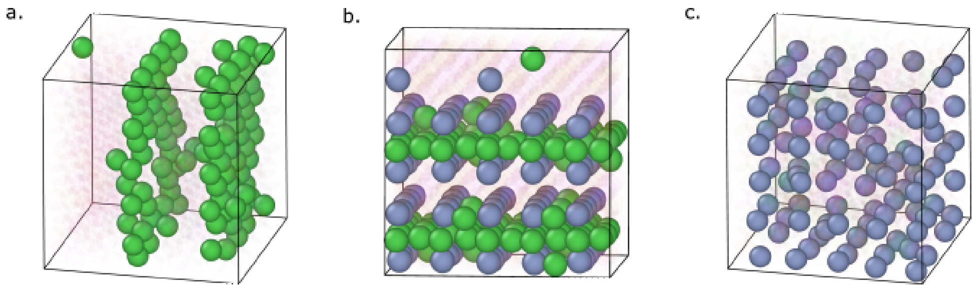


Figure S17. a. Snapshot of CoCrFeMnNi at 300 K, showing all species except Ni transparent, revealing the two Ni(100) planes, b. same snapshot rotated, showing the Ni(100) planes sandwiched by Cr-atoms (blue), and c. snapshot at 720 K with Cr atoms highlighted, revealing Cr order.

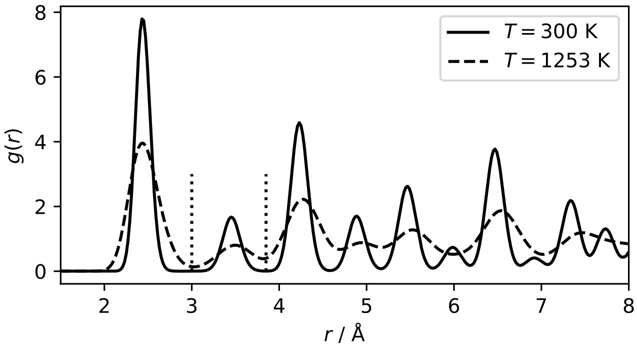


Figure S18. Pair correlation functions computed on the $T = 300$ K (full) and $T = 1253$ K (dashed lines) replicas, averaged over two independent runs of the CoCrFeMnNi system. The vertical dotted lines indicate the regions used in the definition of the pair ordering.

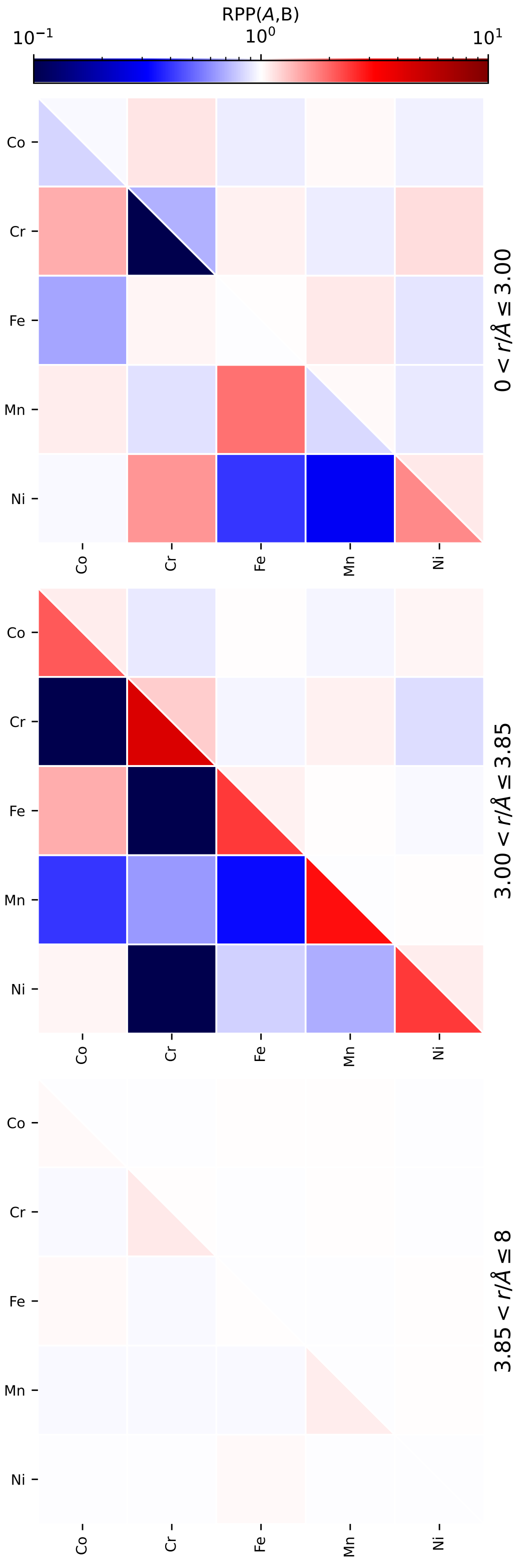


Figure S19. A plot of the relative pair probability for all atom pairs and the three regions corresponding to the first, second, and third peaks in the total pair correlation function (Fig. S18). Each plot shows results for simulations of CoCrFeMnNi at both 300 K (lower-left corner) and 1253 K (top-right corner), averaged over the trajectories and discarding the first 100 ps.

## B. CoCrFeMoNi

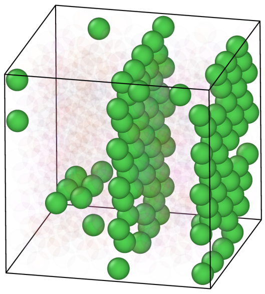

Figure S20. Snapshot of CoCrFeMoNi at 300 K, showing all species except Ni transparent, revealing the two Ni (100) planes.

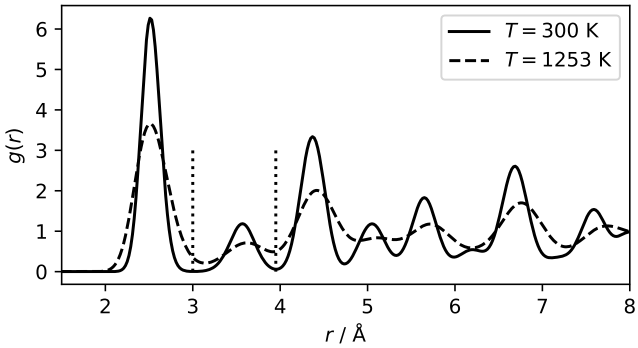


Figure S21. Pair correlation functions computed on the $T$ = 300 K (full) and $T$ = 1253 K (dashed lines) replicas, averaged over the eight independent runs of the CoCrFeMoNi system. The vertical dotted lines indicate the regions used in the definition of the pair ordering.

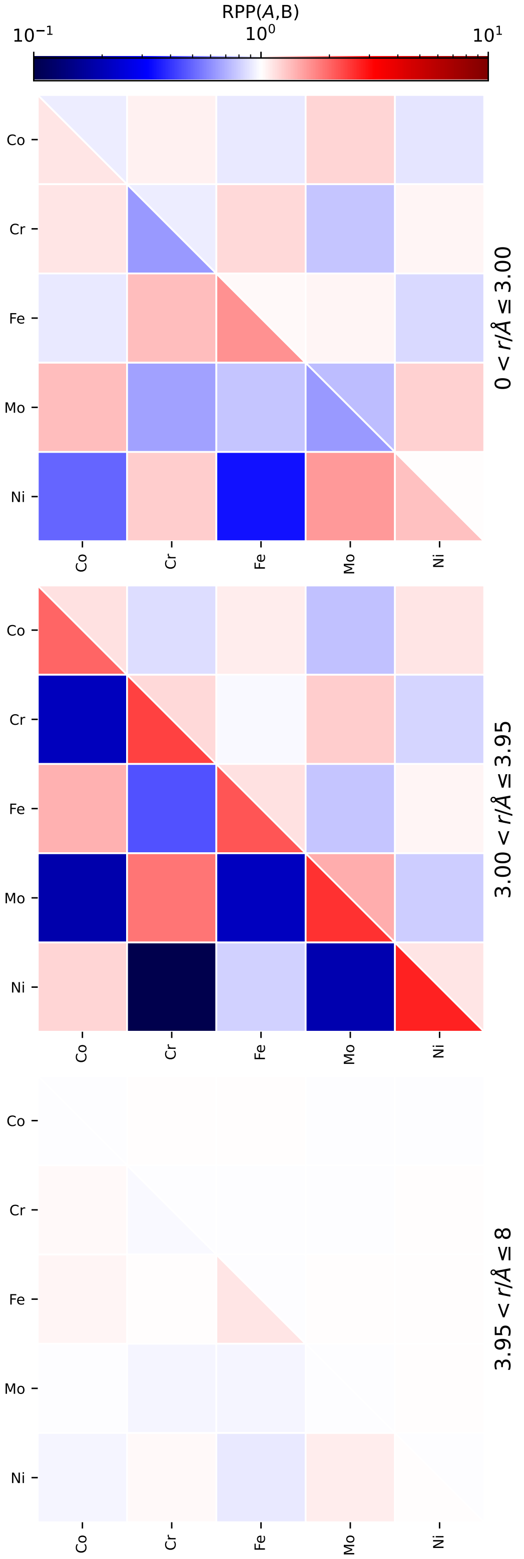


Figure S22. A plot of the relative pair probability for all atom pairs and the three regions corresponding to the first, second, and third peaks in the total pair correlation function (Fig. S21). Each plot shows results for simulations of CoCrFeMoNi at both 300 K (lower-left corner) and 1253 K (top-right corner), averaged over the trajectories and discarding the first 100 ps.

## C. IrPdPtRhRu

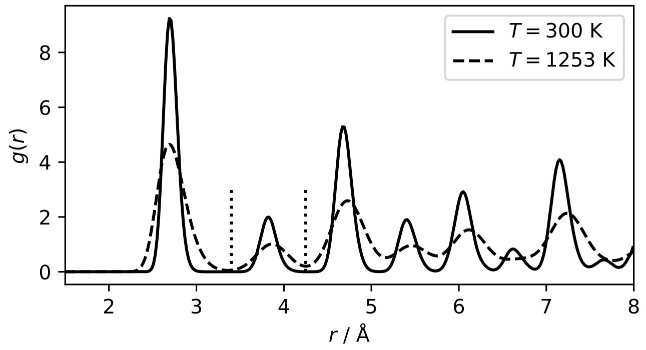


Figure S23. Pair correlation functions computed on the $T = 300$ K (full) and $T = 1253$ K (dashed lines) replicas, averaged over the eight independent runs of the IrPdPtRhRu system. The vertical dotted lines indicate the regions used in the definition of the pair ordering.

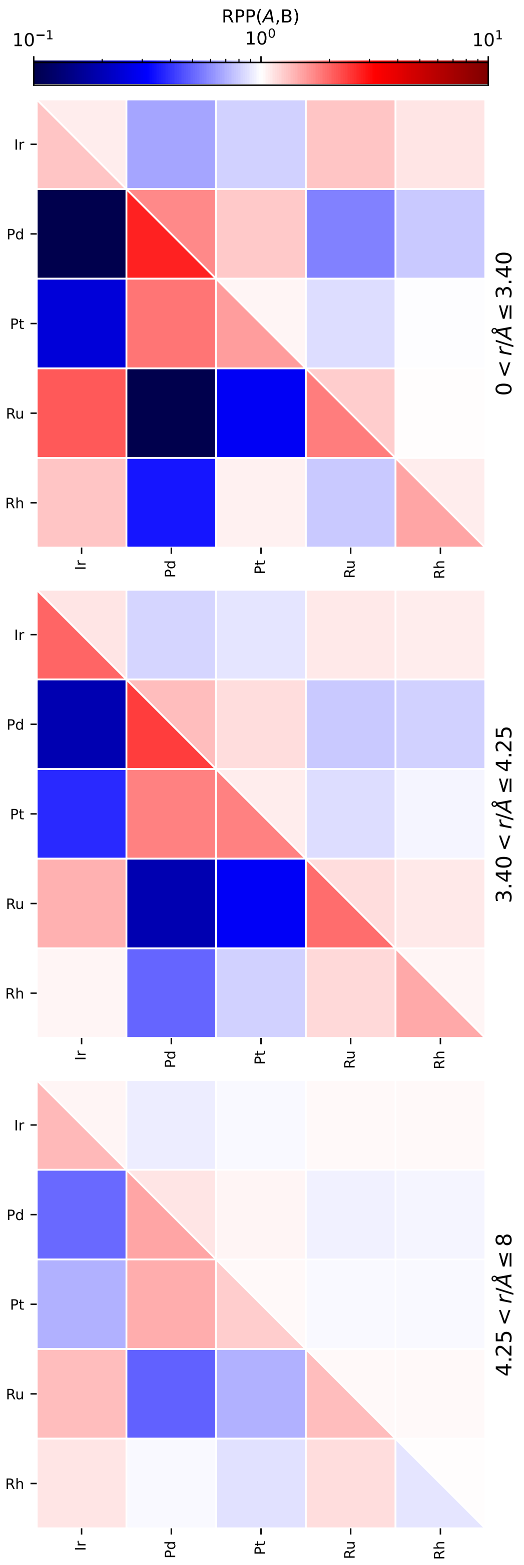


Figure S24. A plot of the relative pair probability for all atom pairs and the three regions corresponding to the first, second, and third peaks in the total pair correlation function (Fig. S21). Each plot shows results for simulations of IrPdPtRhRu at both 300 K (lower-left corner) and 1253 K (top-right corner), averaged over the trajectories and discarding the first 100 ps.

### D. DFT validation of segregation in IrPdPtRuRh

In order to verify that the segregation we observe for IrPdPtRuRh is not an artifact due to the ML model, we ran similar simulations with a smaller supercell containing 180 atoms at 300 K. We performed a simulation with a simple MD trajectory, starting with a random distribution of atoms (random), and one including MC steps (swaps). After equilibration (which led to segregation in the simulation including atom swaps) we extracted 70 snapshots from both the "random" and "swaps" simulations, and re-computed their energies with the same DFT settings we used to generate the train set. It is clear that the energies are in very good agreement. There is a small near-constant shift in energies, but the relative energy of the two sets of configurations, as well as the spread within each subset, are reproduced with an accuracy comparable to that seen in the validation set. The large enthalpy gain associated with ordering is observed also in DFT calculations, which rules out the possibility that the observation of de-mixing is a consequence of errors in the ML model. We estimated the change in de-mixing free-energy due to the ML approximation using a free-energy perturbation expression, finding an error below 3meV/atom.

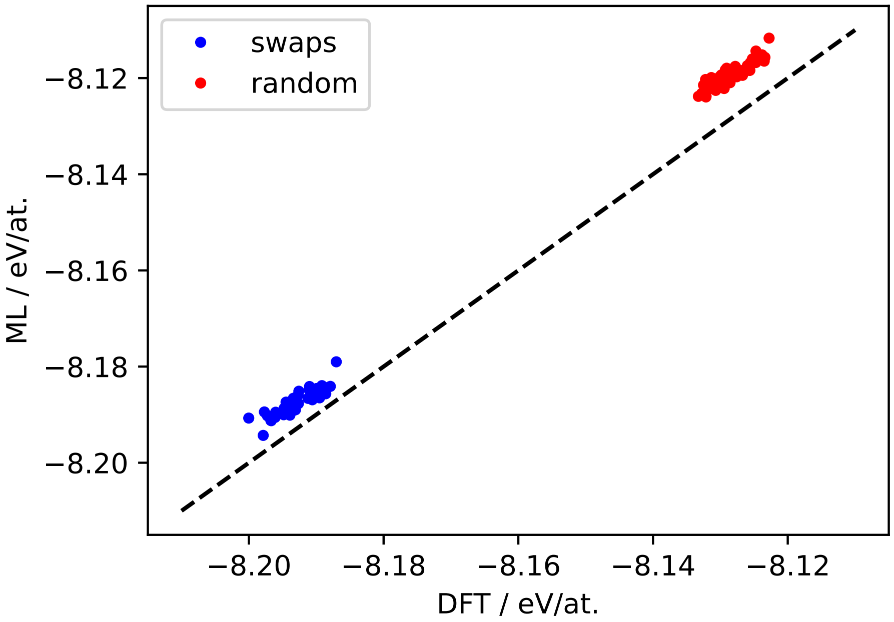


Figure S25. Parity plot of the HEA25-4-NN vs DFT energies for snapshots of a 180-atoms supercell containing IrPdPtRuRh, simulated at 300 K with plain MD (random) and including MC steps (swaps). A plot of the relative pair probability for all atom pairs and the three regions corresponding to the first, second, and third peaks in the total pair correlation function (Fig. S23). Each plot shows results for simulations of IrPdPtRhRu at both 500 K (lower-left corner) and 933 K (top-right corner), averaged over the trajectories and dis- carding the first 100 ps.

## VI. FULL LIST OF HULL PLOTS

Below you can find a full list of convex hull plots, that extend to the full list of 25 elements the plots shown in Fig. S9. Solid lines highlight the hulls obtained from the single-point DFT calculations (blue) and the ML predictions (purple). The dashed line identifies the structures that are stable based on the energies available in the Materials Project database. Note that in many cases there is a qualitative discrepancy not only between the HEA4NN model and the Materials Project reference, but also between the Materials Project reference and the internally-consistent DFT reference. Black points reflect discarded structures based on the distance measure reflecting the similarity to BCC or FCC phases.

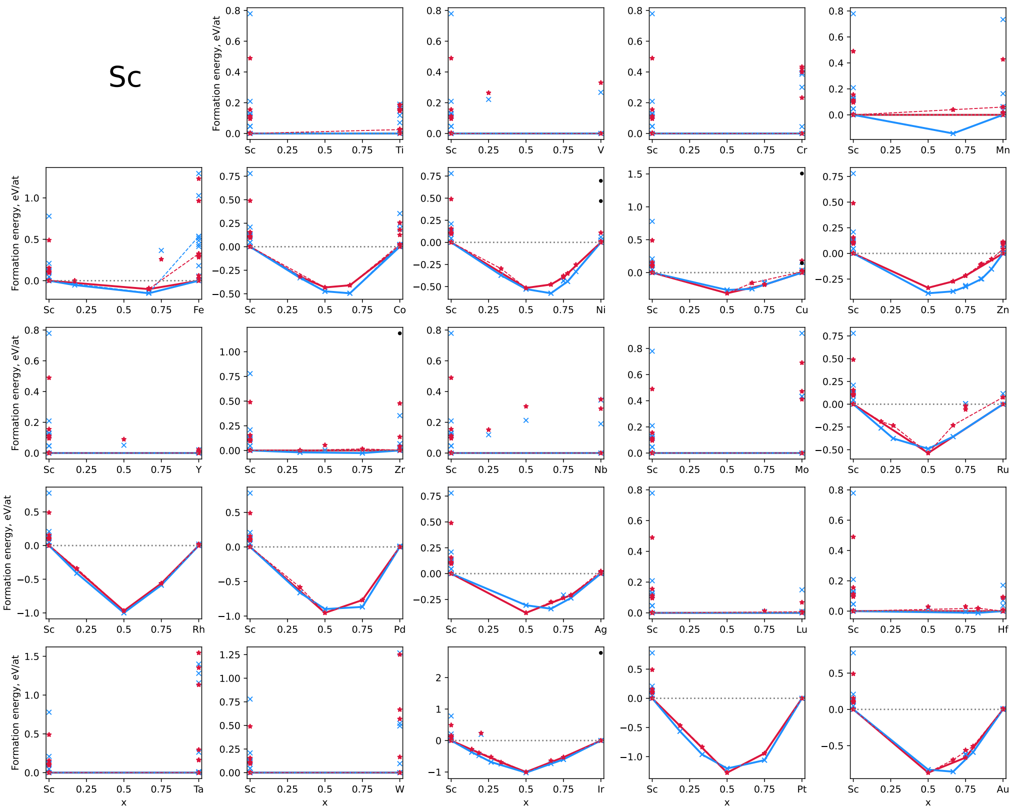


## REFERENCES


[1] G. Kresse and J. Furthmüller, Phys. Rev. B **54**, 11169 (1996).

[2] G. I. Csonka, J. P. Perdew, A. Ruzsinszky, P. H. Philipsen, S. Lebègue, J. Paier, O. A. Vydrov, and J. G. Ángyán, Physical Review B **79**, 155107 (2009).

[3] G. Kresse and D. Joubert, Physical review b **59**, 1758 (1999).

[4] H. J. Monkhorst and J. D. Pack, Phys. Rev. B **13**, 5188 (1976).

[5] M. J. Willatt, F. Musil, and M. Ceriotti, Phys. Chem. Chem. Phys. **20**, 29661 (2018).

[6] C. Chen and S. P. Ong, "A universal graph deep learning interatomic potential for the periodic table," (2022).

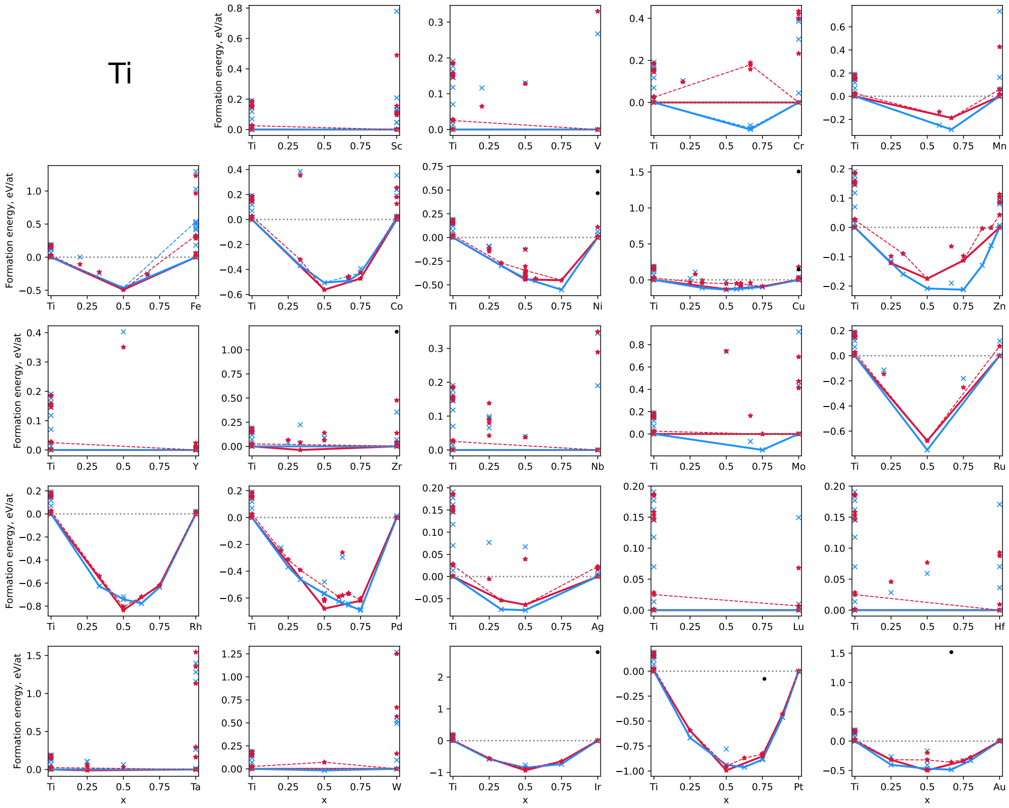
Ti
Formation energy, eV/at
x
Sc
V
Cr
Mn
Fe
Co
Ni
Cu
Zn
Y
Zr
Nb
Mo
Ru
Rh
Pd
Ag
Lu
Hf
Ta
W
Ir
Pt
Au

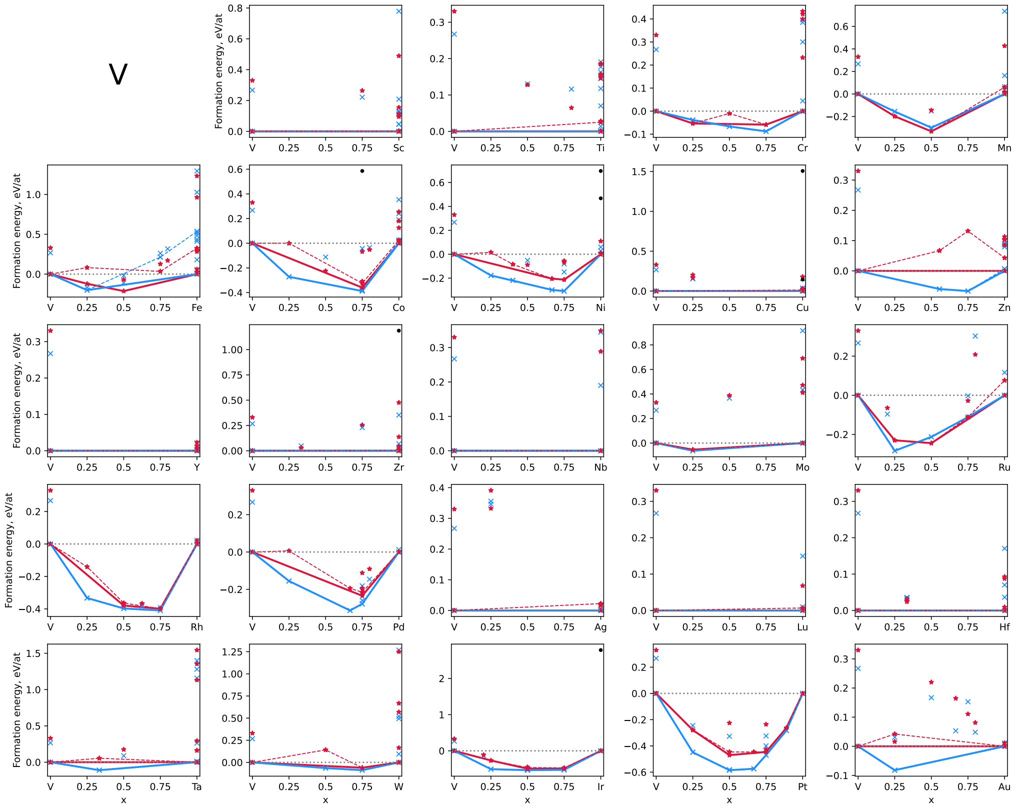
V
Formation energy, eV/at
x
Sc
Ti
Cr
Mn
Fe
Co
Ni
Cu
Zn
Y
Zr
Nb
Mo
Ru
Rh
Pd
Ag
Lu
Hf
Ta
W
Ir
Pt
Au

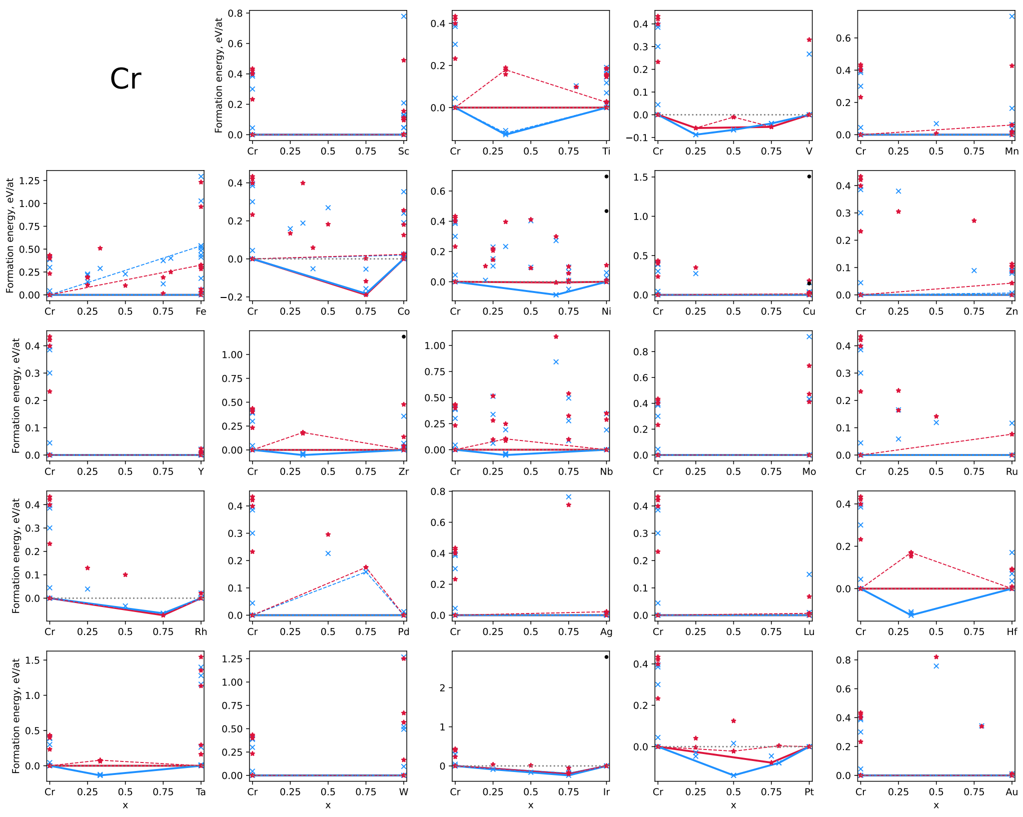
Cr
Formation energy, eV/at
x

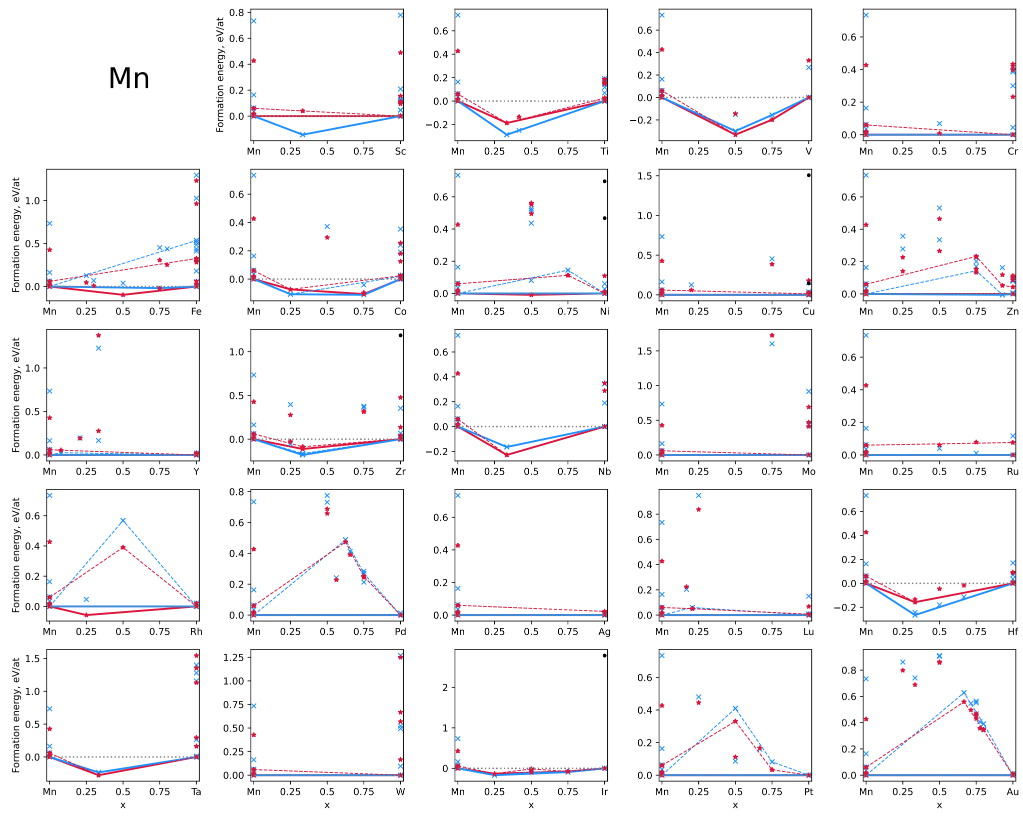
Mn
Formation energy, eV/at
x

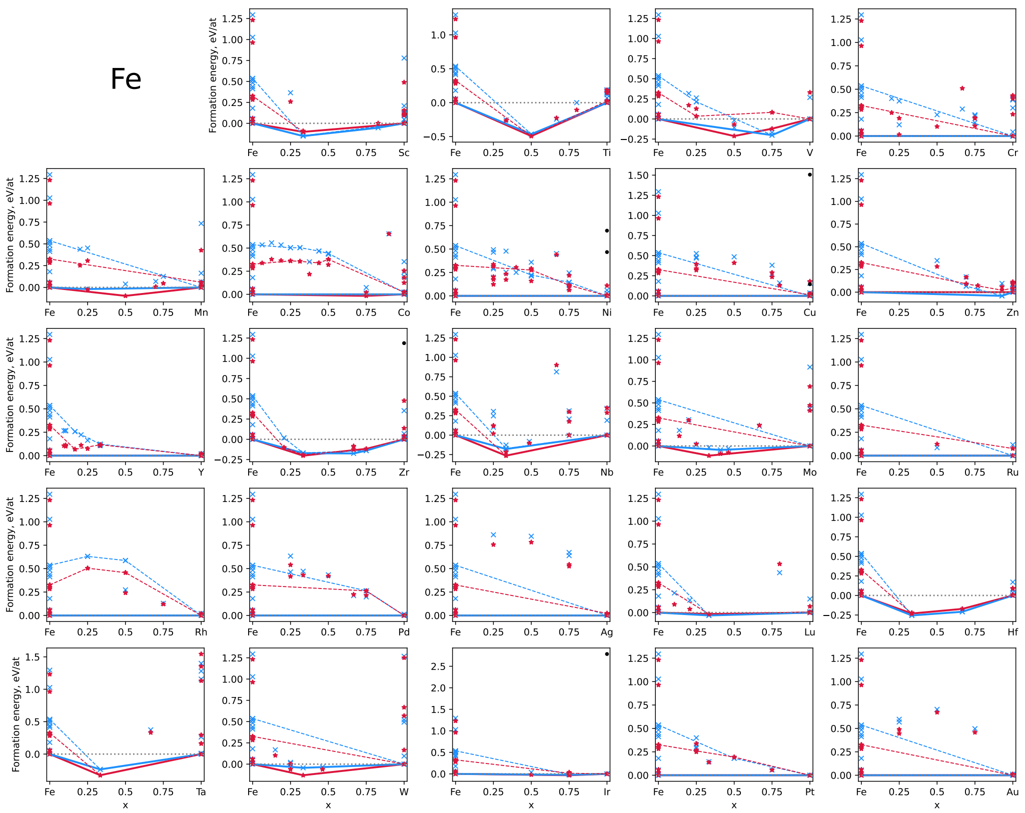
Fe
Formation energy, eV/at
x
Sc Ti V Cr Mn Co Ni Cu Zn Y Zr Nb Mo Ru Rh Pd Ag Lu Hf Ta W Ir Pt Au

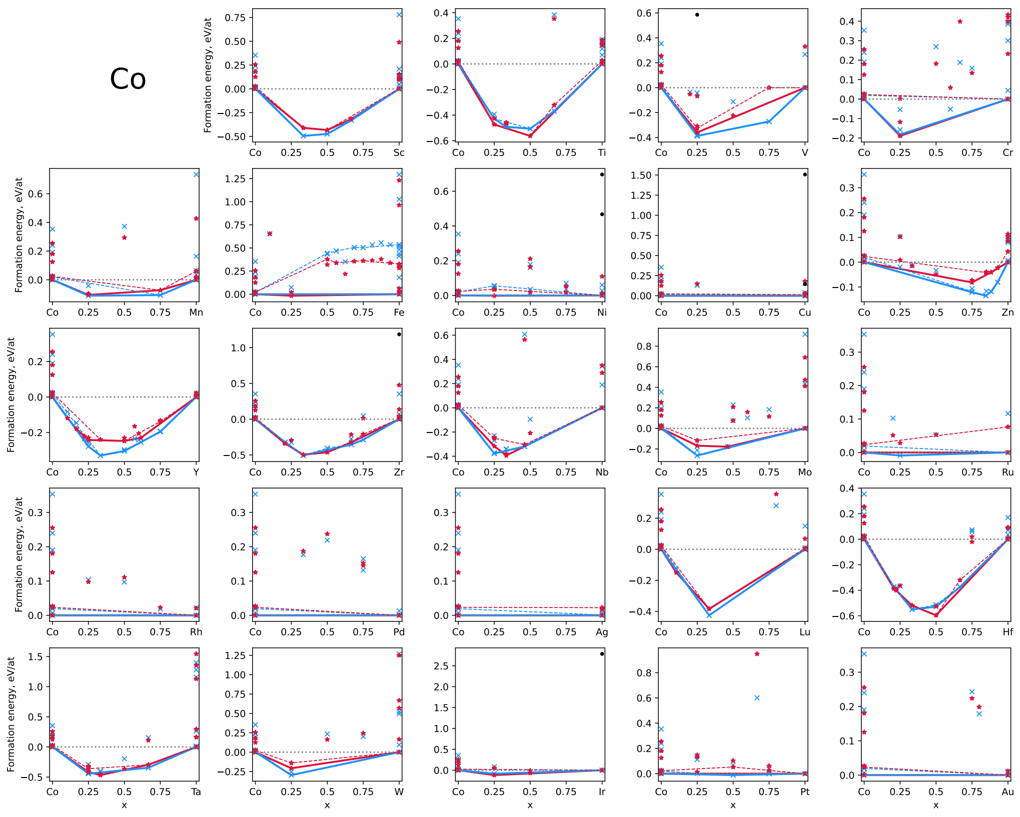
Co
Formation energy, eV/at
x
Sc Ti V Cr Mn Fe Ni Cu Zn Y Zr Nb Mo Ru Rh Pd Ag Lu Hf Ta W Ir Pt Au

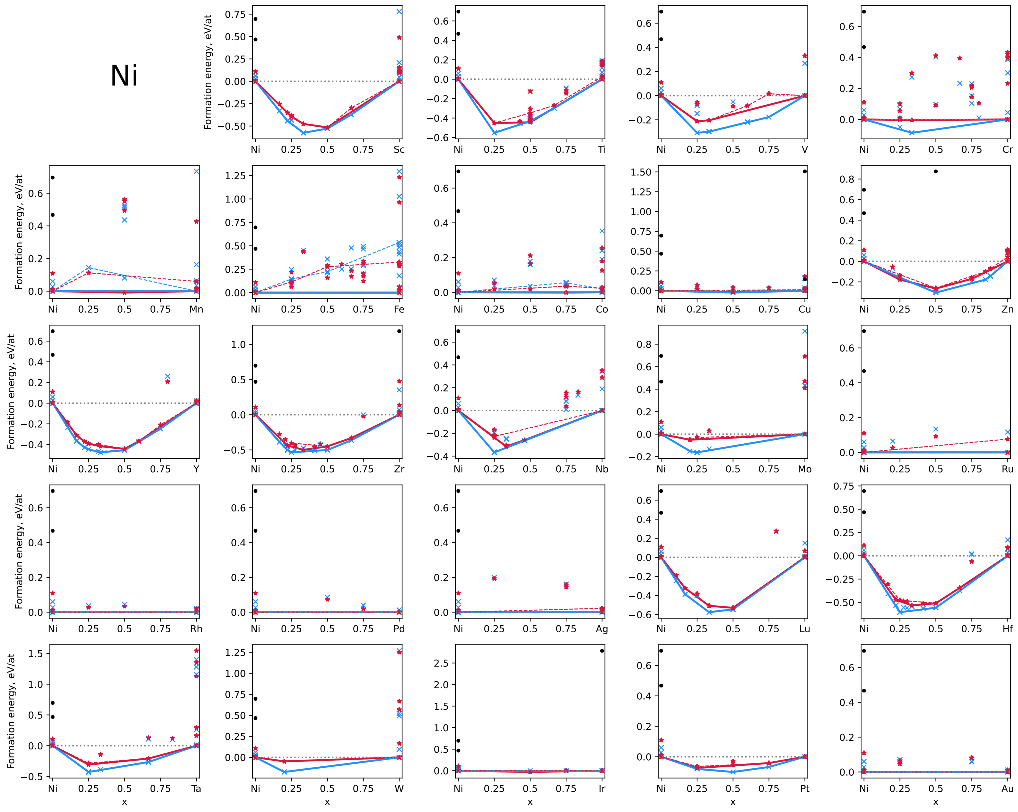
Ni
Formation energy, eV/at
x
Ni Sc Ti V Cr Mn Fe Co Cu Zn Y Zr Nb Mo Ru Rh Pd Ag Lu Hf Ta W Ir Pt Au

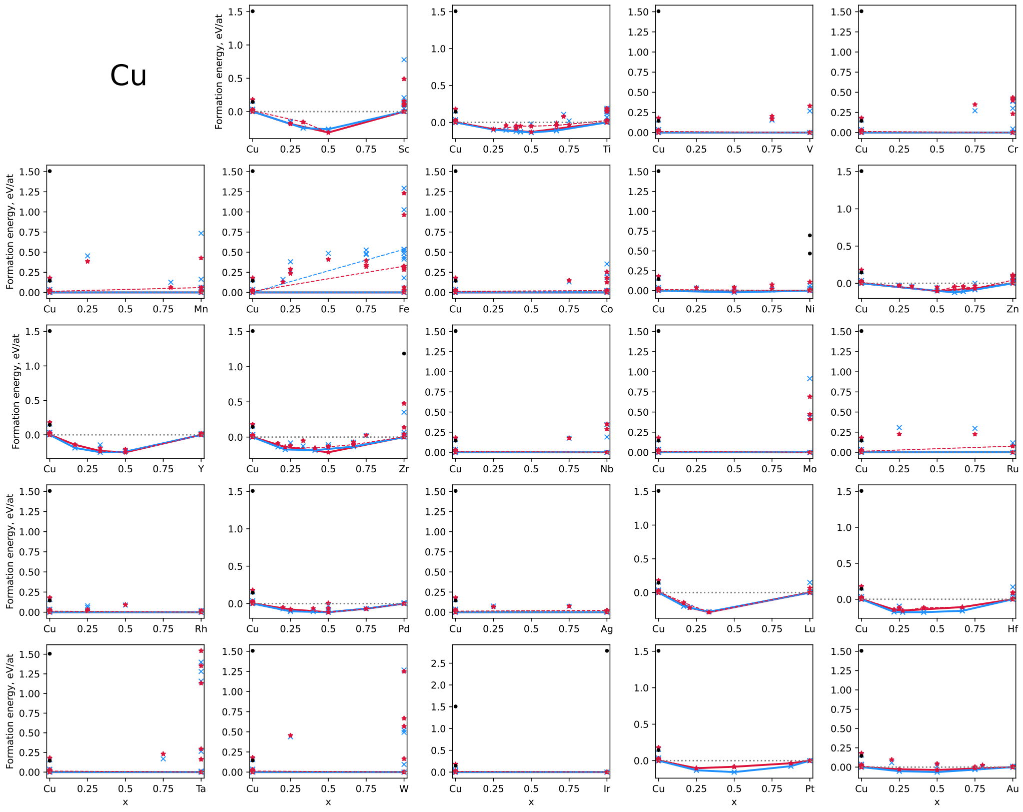
Cu
Formation energy, eV/at
x
Cu Sc Ti V Cr Mn Fe Co Ni Zn Y Zr Nb Mo Ru Rh Pd Ag Lu Hf Ta W Ir Pt Au

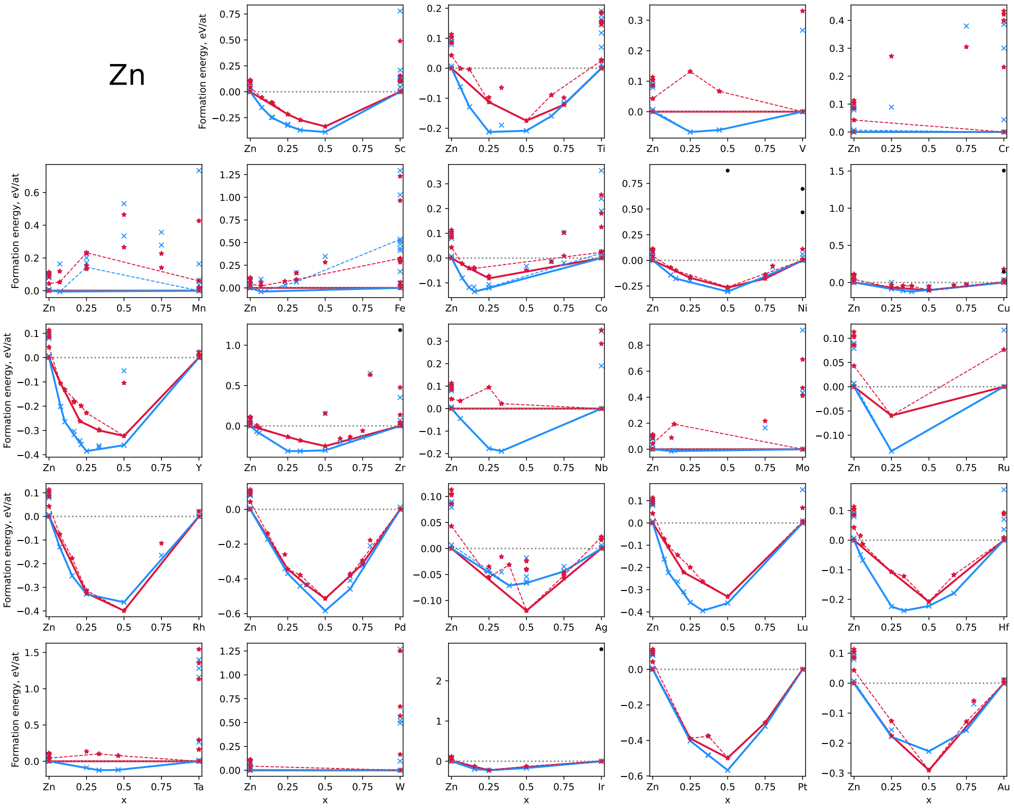
Zn
Formation energy, eV/at
x
Sc Ti V Cr
Mn Fe Co Ni Cu
Y Zr Nb Mo Ru
Rh Pd Ag Lu Hf
Ta W Ir Pt Au

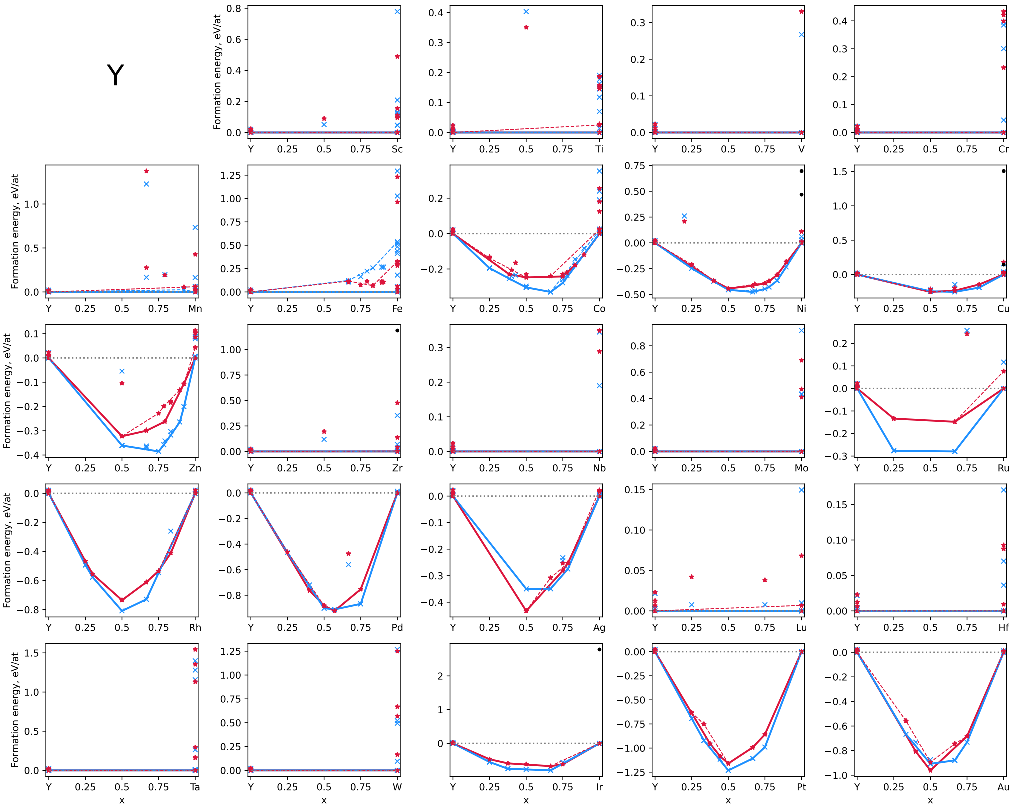
Y
Formation energy, eV/at
x
Sc Ti V Cr
Mn Fe Co Ni Cu
Zn Zr Nb Mo Ru
Rh Pd Ag Lu Hf
Ta W Ir Pt Au

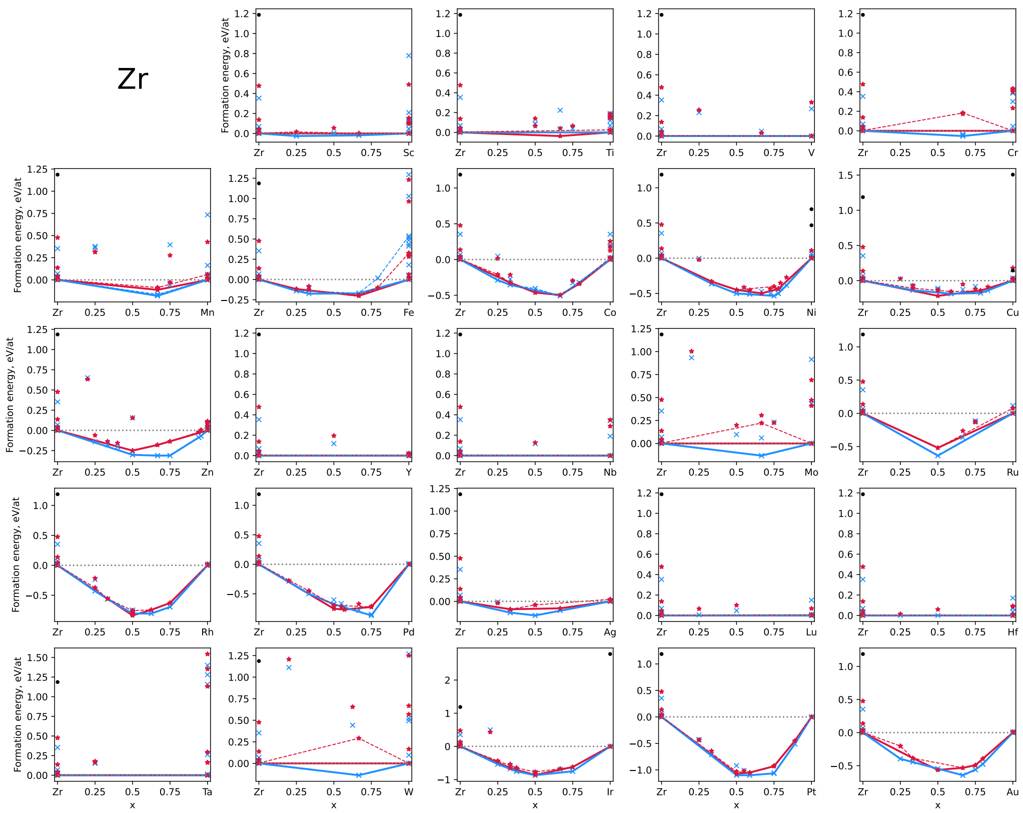
Zr
Formation energy, eV/at
x
Sc
Ti
V
Cr
Mn
Fe
Co
Ni
Cu
Zn
Y
Nb
Mo
Ru
Rh
Pd
Ag
Lu
Hf
Ta
W
Ir
Pt
Au

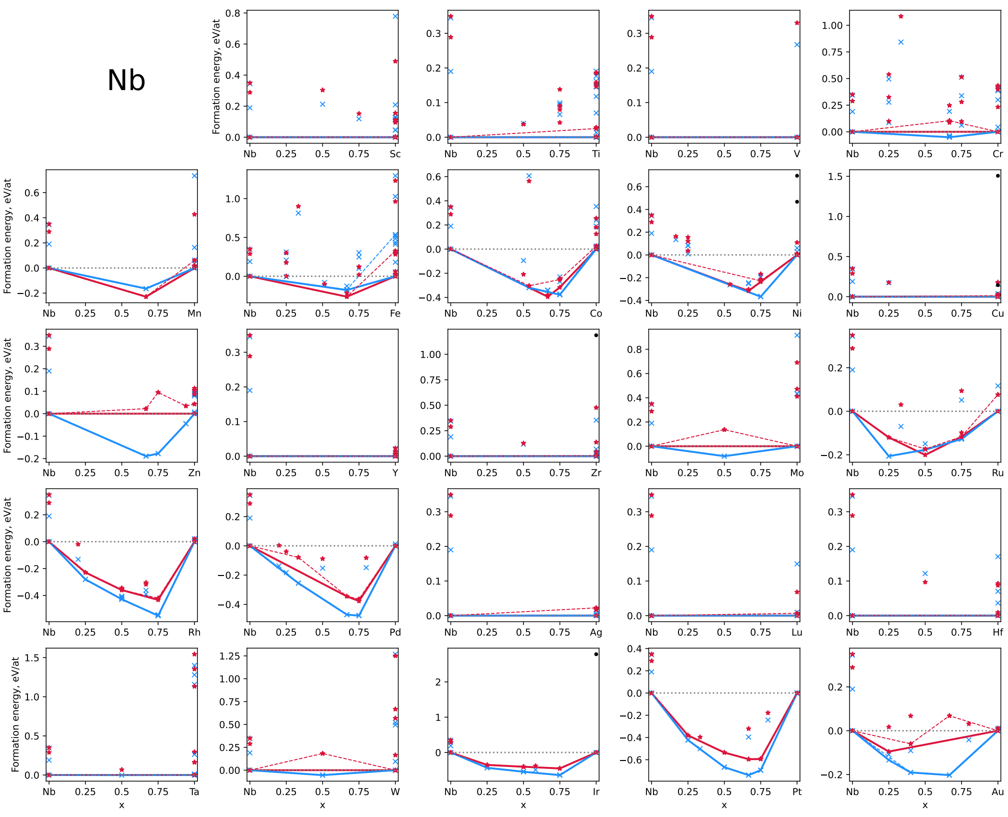
Nb
Formation energy, eV/at
x
Sc
Ti
V
Cr
Mn
Fe
Co
Ni
Cu
Zn
Y
Zr
Mo
Ru
Rh
Pd
Ag
Lu
Hf
Ta
W
Ir
Pt
Au

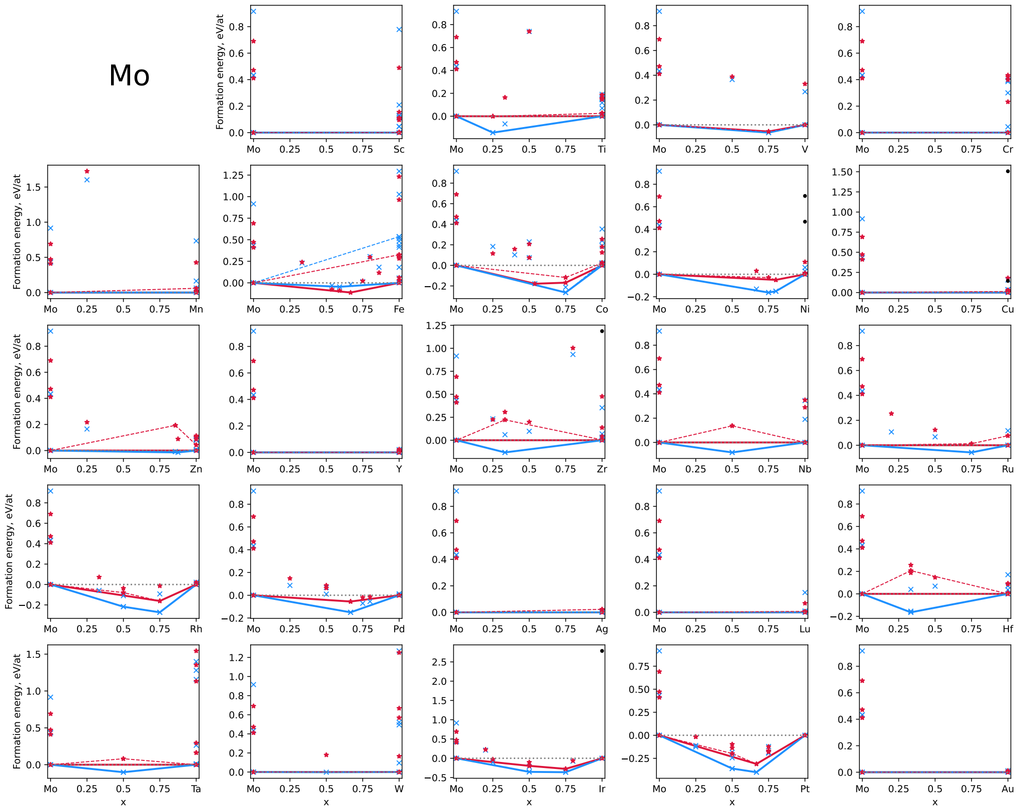
Mo
Formation energy, eV/at
x
Mo
Sc
Ti
V
Cr
Mn
Fe
Co
Ni
Cu
Zn
Y
Zr
Nb
Ru
Rh
Pd
Ag
Lu
Hf
Ta
W
Ir
Pt
Au

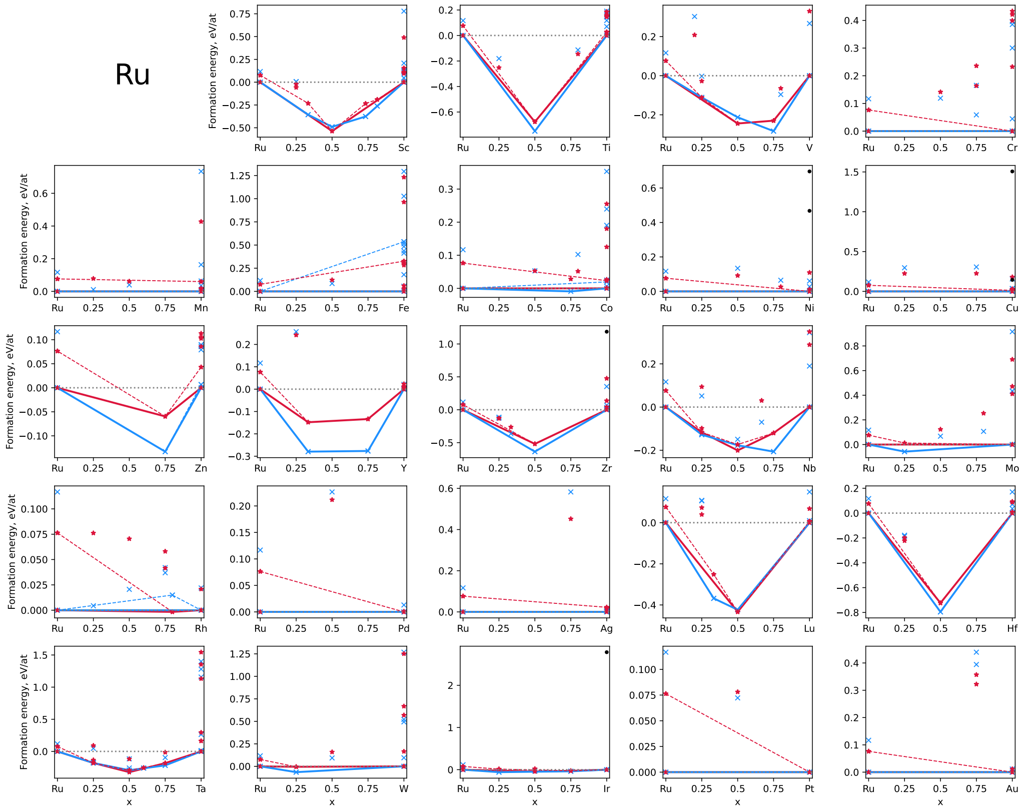
Ru
Formation energy, eV/at
x
Ru
Sc
Ti
V
Cr
Mn
Fe
Co
Ni
Cu
Zn
Y
Zr
Nb
Mo
Rh
Pd
Ag
Lu
Hf
Ta
W
Ir
Pt
Au

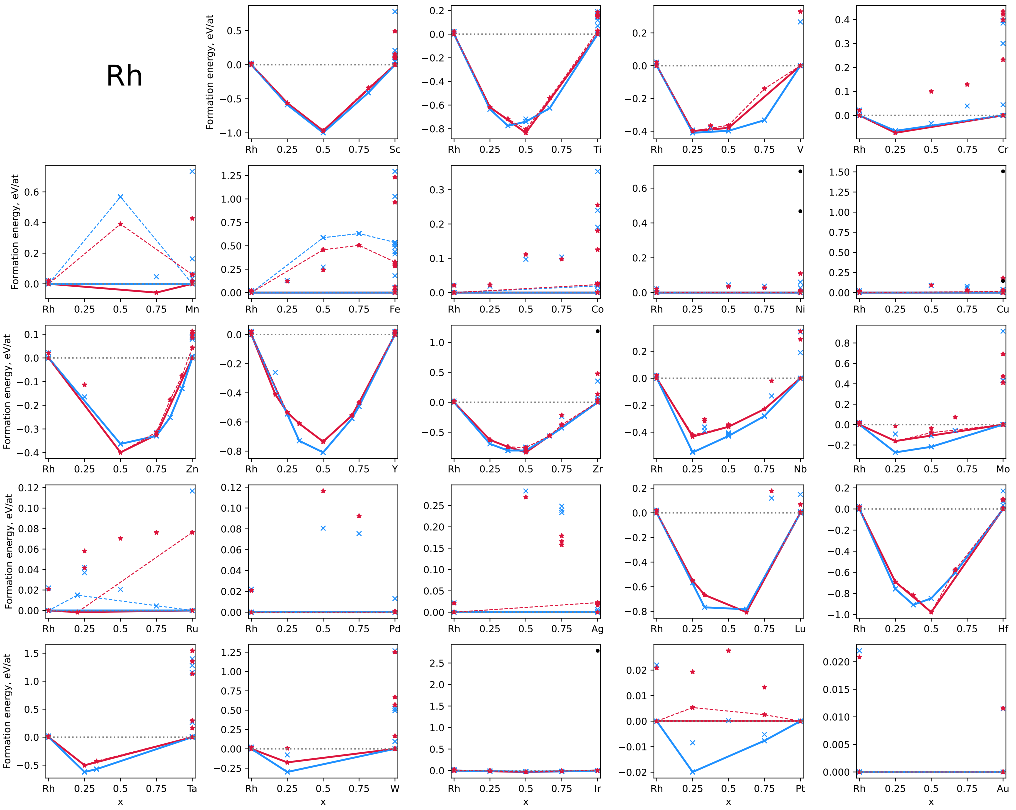
Rh
Formation energy, eV/at
x
Rh
Sc
Ti
V
Cr
Mn
Fe
Co
Ni
Cu
Zn
Y
Zr
Nb
Mo
Ru
Pd
Ag
Lu
Hf
Ta
W
Ir
Pt
Au

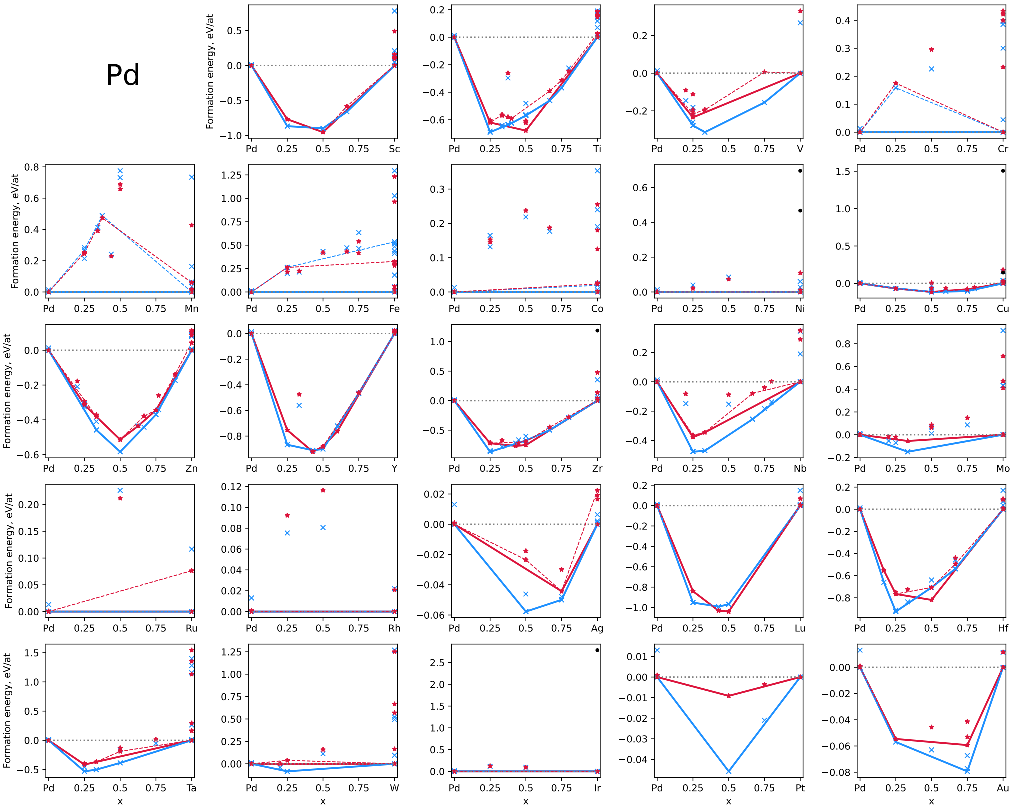
Pd
Formation energy, eV/at
x
Pd
Sc
Ti
V
Cr
Mn
Fe
Co
Ni
Cu
Zn
Y
Zr
Nb
Mo
Ru
Rh
Ag
Lu
Hf
Ta
W
Ir
Pt
Au

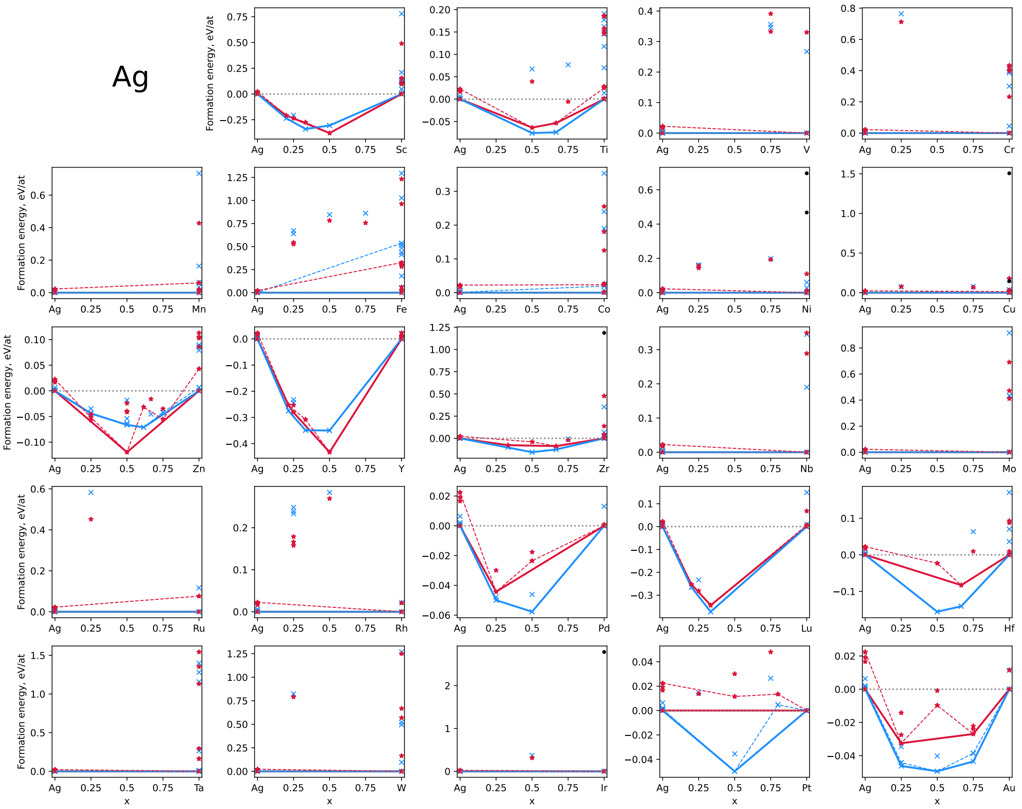
Ag
Formation energy, eV/at
x

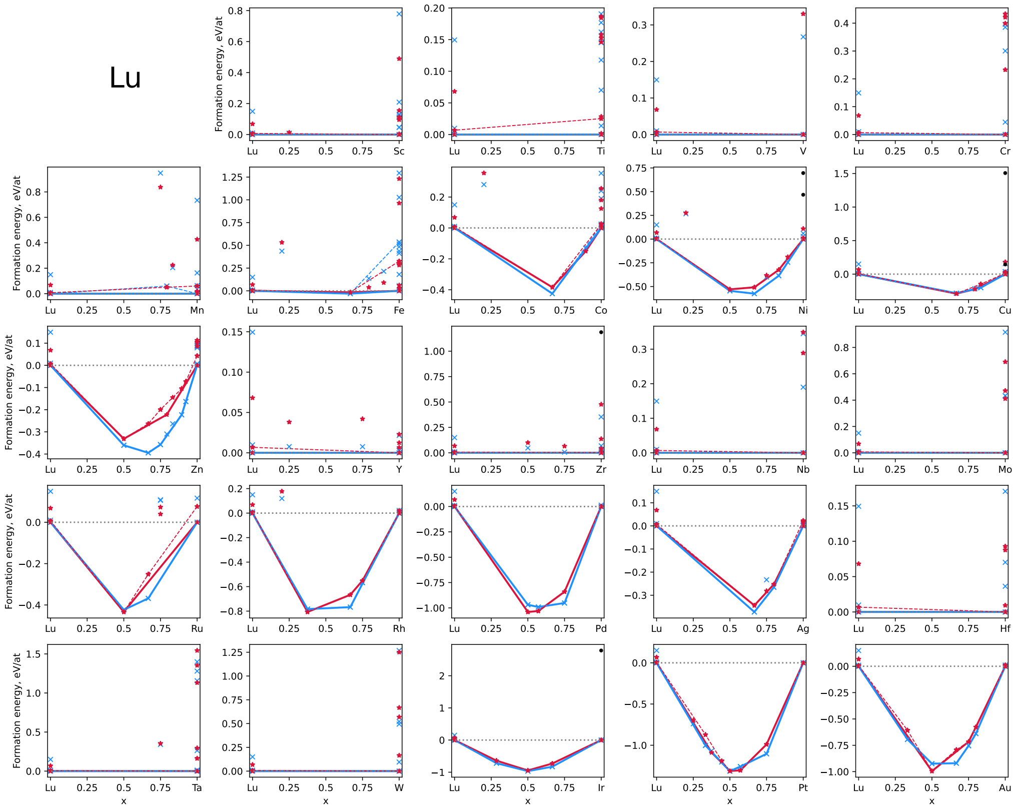
Lu
Formation energy, eV/at
x

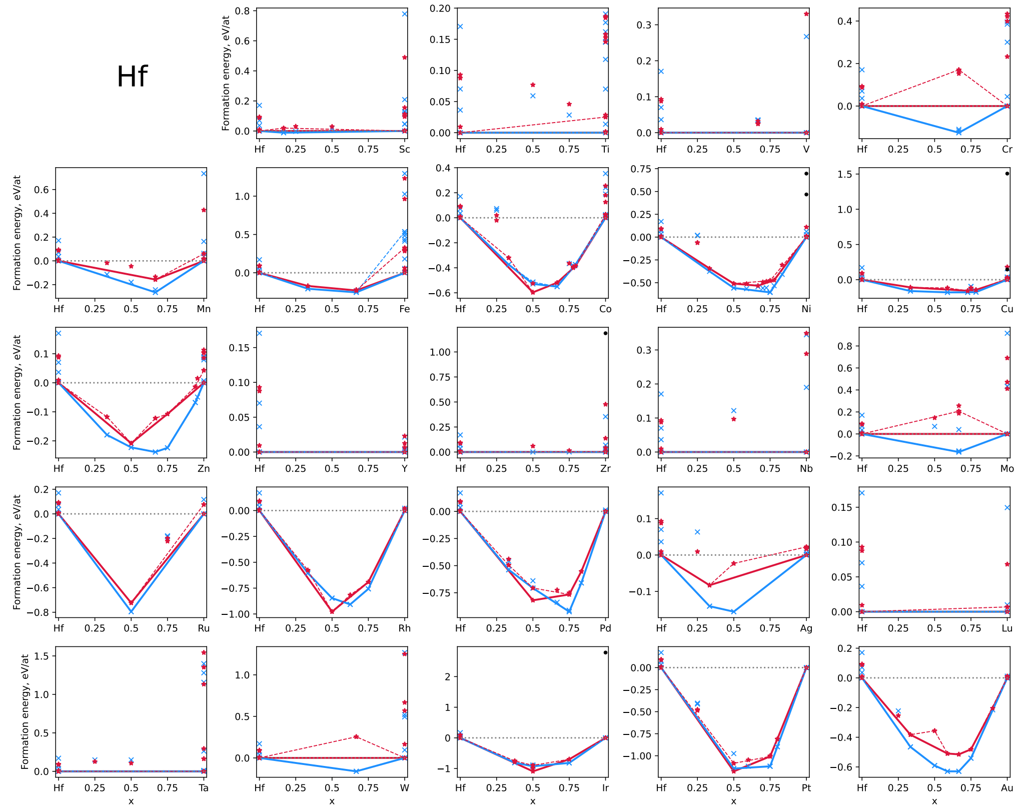
Hf
Formation energy, eV/at
x
Sc
Ti
V
Cr
Mn
Fe
Co
Ni
Cu
Zn
Y
Zr
Nb
Mo
Ru
Rh
Pd
Ag
Lu
Ta
W
Ir
Pt
Au

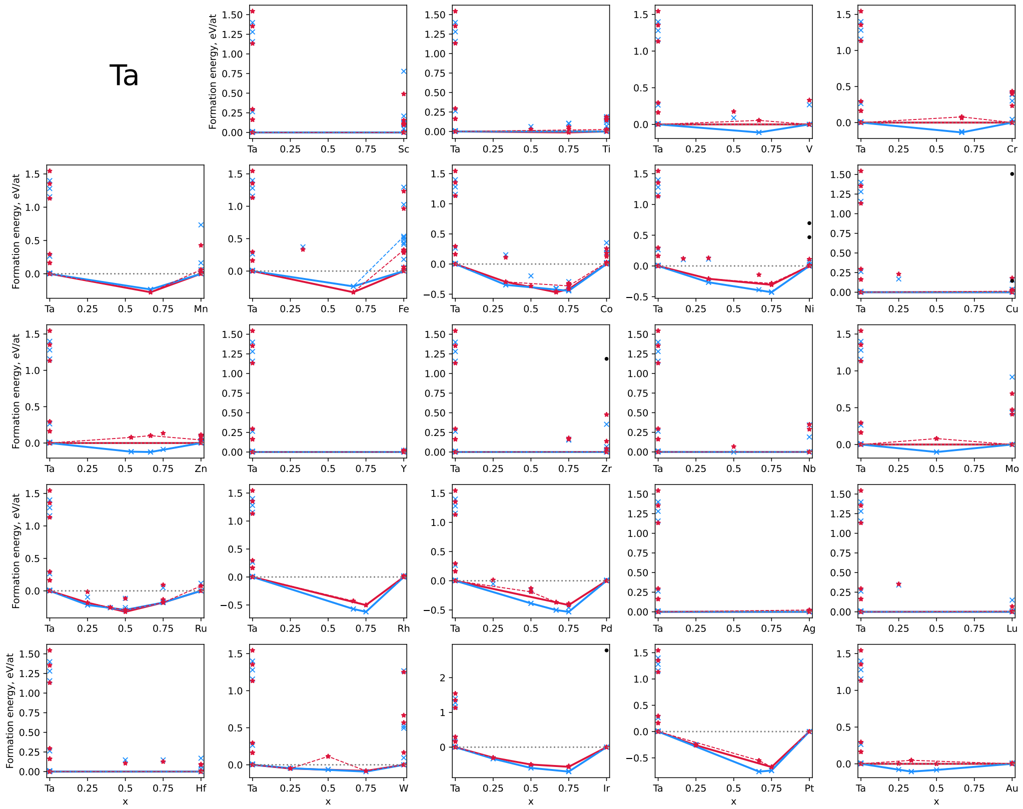
Ta
Formation energy, eV/at
x
Sc
Ti
V
Cr
Mn
Fe
Co
Ni
Cu
Zn
Y
Zr
Nb
Mo
Ru
Rh
Pd
Ag
Lu
Hf
W
Ir
Pt
Au

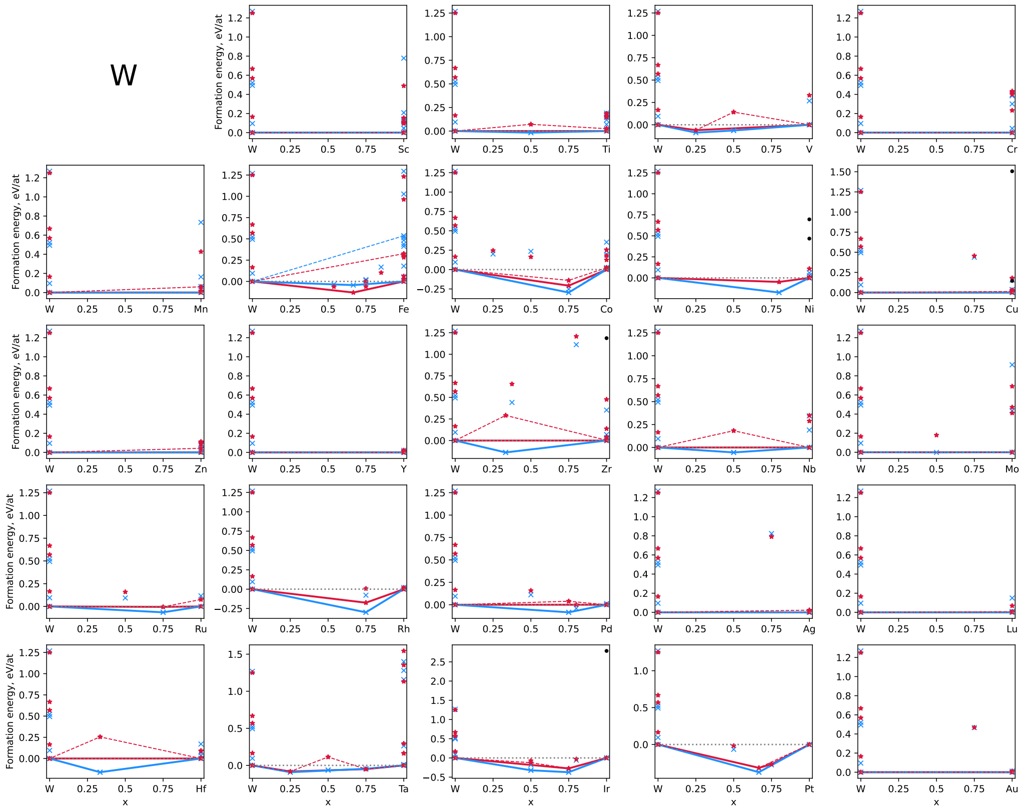
W
Formation energy, eV/at
x
Sc Ti V Cr Mn Fe Co Ni Cu Zn Y Zr Nb Mo Ru Rh Pd Ag Lu Hf Ta Ir Pt Au

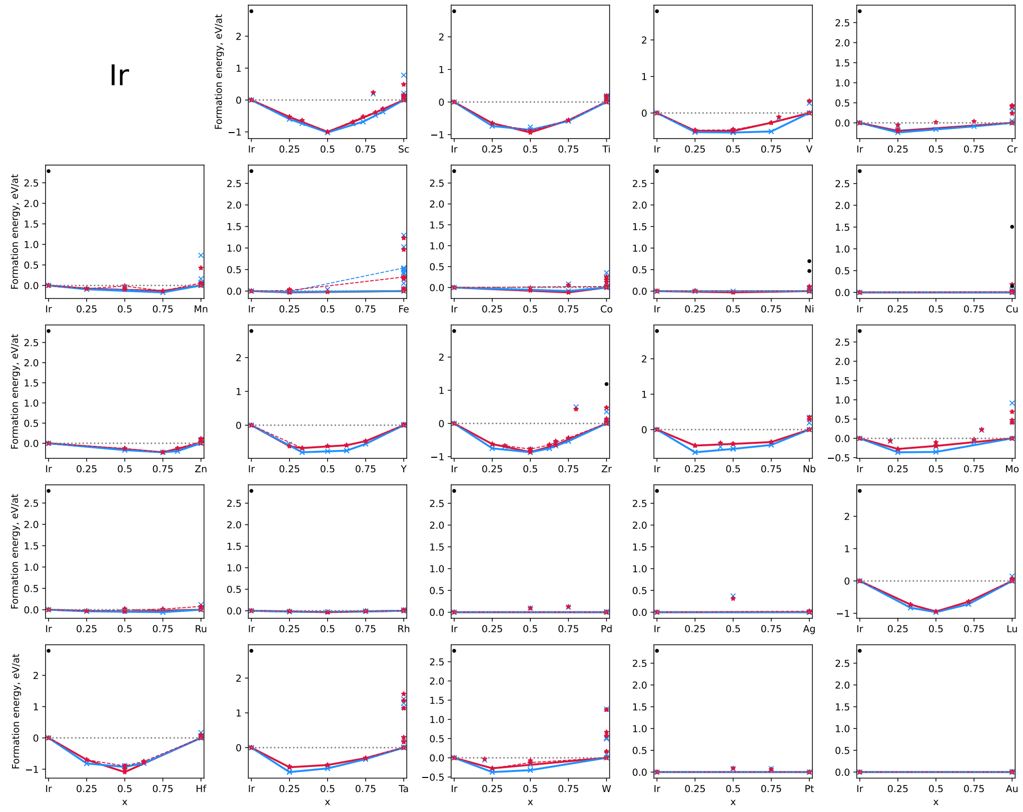
Ir
Formation energy, eV/at
x
Sc Ti V Cr Mn Fe Co Ni Cu Zn Y Zr Nb Mo Ru Rh Pd Ag Lu Hf Ta W Pt Au

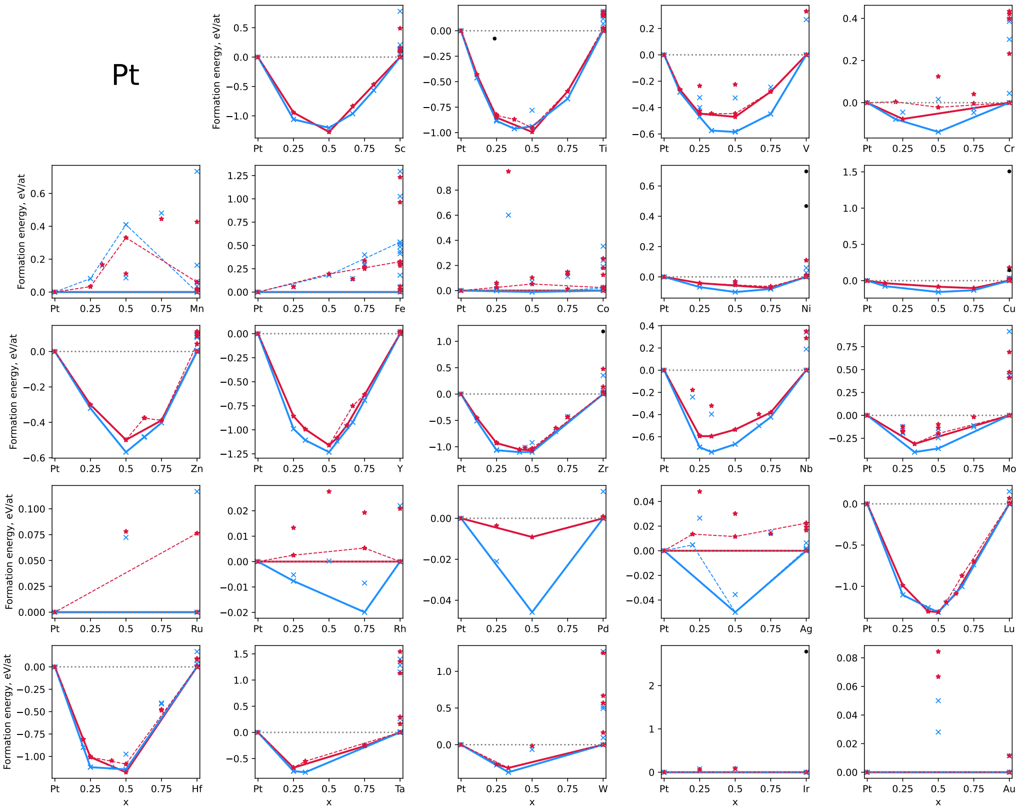
Pt
Formation energy, eV/at
x
Sc
Ti
V
Cr
Mn
Fe
Co
Ni
Cu
Zn
Y
Zr
Nb
Mo
Ru
Rh
Pd
Ag
Lu
Hf
Ta
W
Ir
Au

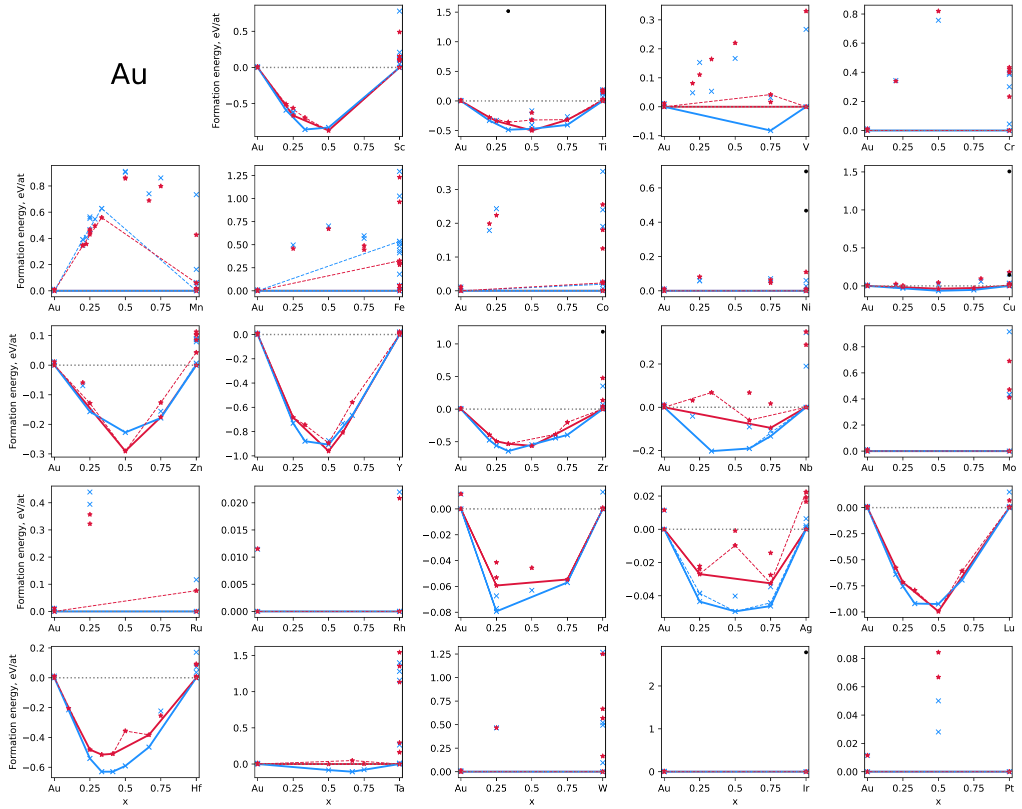
Au
Formation energy, eV/at
x
Sc
Ti
V
Cr
Mn
Fe
Co
Ni
Cu
Zn
Y
Zr
Nb
Mo
Ru
Rh
Pd
Ag
Lu
Hf
Ta
W
Ir
Pt
